# Supplementary material for: N$^3$LO gravitational spin-orbit coupling at order $G^4$
Source: arXiv:2003.02827 source file (2021-07-19)
Supplement: Supplementary file 1 [file appendix.pdf]

## A Graph values

$$\text{Fig. 5(a1.1)} = 2\left(\frac{G^4}{r^5}\frac{\vec{S}_1}{m_1}\cdot\ \vec{v}_2\times\vec{n}\,m_1^3m_2^2\right), \tag{A.1}$$

$$\text{Fig. 5(a1.2)} = 8\left(\frac{G^4}{r^5}\frac{\vec{S}_1}{m_1}\cdot\ \vec{v}_2\times\vec{n}\,m_1^2m_2^3\right), \tag{A.2}$$

$$\text{Fig. 5(a1.3)} = 8\left(\frac{G^4}{r^5}\frac{\vec{S}_1}{m_1}\cdot\ \vec{v}_2\times\vec{n}\,m_1^2m_2^3\right), \tag{A.3}$$

$$\text{Fig. 5(a1.4)} = 8\left(\frac{G^4}{r^5}\frac{\vec{S}_1}{m_1}\cdot\ \vec{v}_2\times\vec{n}\,m_1^3m_2^2\right), \tag{A.4}$$

$$\text{Fig. 5(a1.5)} = -2\left(\frac{G^4}{r^5}\frac{\vec{S}_1}{m_1}\cdot\ \vec{v}_1\times\vec{n}\,m_1^3m_2^2\right), \tag{A.5}$$

$$\text{Fig. 5(a2.1)} = 32\left(\frac{G^4}{r^5}\frac{\vec{S}_1}{m_1}\cdot\ \vec{v}_2\times\vec{n}\,m_1^2m_2^3\right), \tag{A.6}$$

$$\text{Fig. 5(a2.2)} = 16\left(\frac{G^4}{r^5}\frac{\vec{S}_1}{m_1}\cdot\ \vec{v}_2\times\vec{n}\,m_1^2m_2^3\right), \tag{A.7}$$

$$\text{Fig. 5(a2.3)} = 2\left(\frac{G^4}{r^5}\frac{\vec{S}_1}{m_1}\cdot\ \vec{v}_2\times\vec{n}\,m_1^3m_2^2\right), \tag{A.8}$$

$$\text{Fig. 5(a2.4)} = 4\left(\frac{G^4}{r^5}\frac{\vec{S}_1}{m_1}\cdot\ \vec{v}_2\times\vec{n}\,m_1^3m_2^2\right), \tag{A.9}$$

$$\text{Fig. 5(a2.5)} = 4\left(\frac{G^4}{r^5}\frac{\vec{S}_1}{m_1}\cdot\ \vec{v}_2\times\vec{n}\,m_1^3m_2^2\right), \tag{A.10}$$

$$\text{Fig. 5(a2.6)} = \left(\frac{G^4}{r^5}\frac{\vec{S}_1}{m_1}\cdot\ \vec{v}_2\times\vec{n}\,m_1^2m_2^3\right), \tag{A.11}$$

$$\text{Fig. 5(a2.7)} = -2\left(\frac{G^4}{r^5}\frac{\vec{S}_1}{m_1}\cdot\ \vec{v}_1\times\vec{n}\,m_1^3m_2^2\right), \tag{A.12}$$

$$\text{Fig. 5(a2.8)} = -\left(\frac{G^4}{r^5}\frac{\vec{S}_1}{m_1}\cdot\ \vec{v}_1\times\vec{n}\,m_1^2m_2^3\right), \tag{A.13}$$

$$\text{Fig. 5(a3.1)} = \frac{1}{3}\left(\frac{G^4}{r^5}\ \frac{\vec{S}_1}{m_1}\cdot\vec{v}_2\times\vec{n}\,m_1^4m_2\right), \tag{A.14}$$

$$\text{Fig. 5(a3.2)} = \frac{64}{3}\left(\frac{G^4}{r^5}\ \frac{\vec{S}_1}{m_1}\cdot\vec{v}_2\times\vec{n}\,m_1m_2^4\right), \tag{A.15}$$

$$\text{Fig. 5(a3.3)} = -\frac{1}{3}\left(\frac{G^4}{r^5}\ \frac{\vec{S}_1}{m_1}\cdot\vec{v}_1\times\vec{n}\,m_1^4m_2\right), \tag{A.16}$$

$$\text{Fig. 5(b1.1)} = -32\left(\frac{G^4}{r^5}\frac{\vec{S}_1}{m_1}\cdot\ \vec{v}_2\times\vec{n}\,m_1^2m_2^3\right), \tag{A.17}$$

$$\text{Fig. 5(b1.2)} = -32\left(\frac{G^4}{r^5}\frac{\vec{S}_1}{m_1}\cdot\ \vec{v}_2\times\vec{n}\,m_1^2m_2^3\right), \tag{A.18}$$

$$\text{Fig. 5(b1.3)} = -2\left(\frac{G^4}{r^5}\frac{\vec{S}_1}{m_1}\cdot\ \vec{v}_2\times\vec{n}\,m_1^3m_2^2\right), \tag{A.19}$$

$$\text{Fig. 5(b1.4)} = -8\left(\frac{G^4}{r^5}\frac{\vec{S}_1}{m_1}\cdot\ \vec{v}_2\times\vec{n}\,m_1^3m_2^2\right), \tag{A.20}$$

$$\text{Fig. 5(b1.5)} = 2\left(\frac{G^4}{r^5}\frac{\vec{S}_1}{m_1}\cdot\ \vec{v}_1\times\vec{n}\,m_1^3m_2^2\right), \tag{A.21}$$

$$\text{Fig. 5(b1.6)} = 8\left(\frac{G^4}{r^5}\frac{\vec{S}_1}{m_1}\cdot\ \vec{v}_1\times\vec{n}\,m_1^3m_2^2\right), \tag{A.22}$$

$$\text{Fig. 5(b1.7)} = 2\left(\frac{G^4}{r^5}\frac{\vec{S}_1}{m_1}\cdot\ \vec{v}_1\times\vec{n}\,m_1^2m_2^3\right), \tag{A.23}$$

$$\text{Fig. 5(b1.8)} = 2\left(\frac{G^4}{r^5}\frac{\vec{S}_1}{m_1}\cdot\ \vec{v}_2\times\vec{n}\,m_1^2m_2^3\right), \tag{A.24}$$

$$\text{Fig. 5(b1.9)} = -\frac{1}{2}\left(\frac{G^4}{r^5}\ \frac{\vec{S}_1}{m_1}\cdot\vec{v}_1\times\vec{n}\,m_1^3\ m_2^2\right), \tag{A.25}$$

$$\text{Fig. 5(b1.10)} = -8\left(\frac{G^4}{r^5}\ \frac{\vec{S}_1}{m_1}\cdot\vec{v}_1\times\vec{n}\,m_1^3\ m_2^2\right), \tag{A.26}$$

$$\text{Fig. 5(b1.11)} = 0, \tag{A.27}$$

$$\text{Fig. 5(b1.12)} = 4\left(\frac{G^4}{r^5}\ \frac{\vec{S}_1}{m_1}\cdot\vec{v}_2\times\vec{n}\,m_1^2\ m_2^3\right), \tag{A.28}$$

$$\text{Fig. 5(b1.13)} = 2\left(\frac{G^4}{r^5}\ \frac{\vec{S}_1}{m_1}\cdot\vec{v}_1\times\vec{n}\,m_1^3\ m_2^2\right), \tag{A.29}$$

$$\text{Fig. 5(b1.14)} = \frac{1}{2}\left(\frac{G^4}{r^5}\ \frac{\vec{S}_1}{m_1}\cdot\vec{v}_1\times\vec{n}\,m_1^3\ m_2^2\right), \tag{A.30}$$

$$\text{Fig. 5(b2.1)} = -8\left(\frac{G^4}{r^5}\ \frac{\vec{S}_1}{m_1}\cdot\vec{v}_2\times\vec{n}\,m_1^3\ m_2^2\right), \tag{A.31}$$

$$\text{Fig. 5(b2.2)} = -8\left(\frac{G^4}{r^5}\ \frac{\vec{S}_1}{m_1}\cdot\vec{v}_2\times\vec{n}\,m_1^2\ m_2^3\right), \tag{A.32}$$

$$\text{Fig. 5(b2.3)} = 8\left(\frac{G^4}{r^5}\ \frac{\vec{S}_1}{m_1}\cdot\vec{v}_1\times\vec{n}\,m_1^2\ m_2^3\right), \tag{A.33}$$

$$\text{Fig. 5(b2.4)} = -\frac{1}{2}\left(\frac{G^4}{r^5}\ \frac{\vec{S}_1}{m_1}\cdot\vec{v}_1\times\vec{n}\,m_1^3\ m_2^2\right), \tag{A.34}$$

$$\text{Fig. 5(b2.5)} = -8\left(\frac{G^4}{r^5}\;\frac{\vec{S}_1}{m_1}\cdot\vec{v}_1\times\vec{n}\,m_1^2\;m_2^3\right), \tag{A.35}$$

$$\text{Fig. 5(b2.6)} = 0, \tag{A.36}$$

$$\text{Fig. 5(b2.7)} = \frac{1}{2}\;\left(\frac{G^4}{r^5}\frac{\vec{S}_1}{m_1}\cdot\;\vec{v}_2\times\vec{n}\,m_1^3m_2^2\right), \tag{A.37}$$

$$\text{Fig. 5(b2.8)} = 2\left(\frac{G^4}{r^5}\frac{\vec{S}_1}{m_1}\cdot\;\vec{v}_1\times\vec{n}\,m_1^2m_2^3\right), \tag{A.38}$$

$$\text{Fig. 5(b3.1)} = -32\left(\frac{G^4}{r^5}\frac{\vec{S}_1}{m_1}\cdot\;\vec{v}_2\times\vec{n}\,m_1^2m_2^3\right), \tag{A.39}$$

$$\text{Fig. 5(b3.2)} = -2\left(\frac{G^4}{r^5}\frac{\vec{S}_1}{m_1}\cdot\;\vec{v}_2\times\vec{n}\,m_1^3m_2^2\right), \tag{A.40}$$

$$\text{Fig. 5(b3.3)} = 2\left(\frac{G^4}{r^5}\frac{\vec{S}_1}{m_1}\cdot\;\vec{v}_1\times\vec{n}\,m_1^3m_2^2\right), \tag{A.41}$$

$$\text{Fig. 5(b3.4)} = \left(\frac{G^4}{r^5}\frac{\vec{S}_1}{m_1}\cdot\;\vec{v}_1\times\vec{n}\,m_1^2m_2^3\right), \tag{A.42}$$

$$\text{Fig. 5(b3.5)} = \left(\frac{G^4}{r^5}\frac{\vec{S}_1}{m_1}\cdot\;\vec{v}_2\times\vec{n}\,m_1^2m_2^3\right), \tag{A.43}$$

$$\text{Fig. 5(b3.6)} = -\frac{1}{2}\left(\frac{G^4}{r^5}\;\frac{\vec{S}_1}{m_1}\cdot\vec{v}_1\times\vec{n}\,m_1^3\;m_2^2\right), \tag{A.44}$$

$$\text{Fig. 5(b3.7)} = 2\left(\frac{G^4}{r^5}\;\frac{\vec{S}_1}{m_1}\cdot\vec{v}_2\times\vec{n}\,m_1^2\;m_2^3\right), \tag{A.45}$$

$$\text{Fig. 5(b3.8)} = \frac{1}{2}\left(\frac{G^4}{r^5}\;\frac{\vec{S}_1}{m_1}\cdot\vec{v}_1\times\vec{n}\,m_1^3\;m_2^2\right), \tag{A.46}$$

$$\text{Fig. 5(b4.1)} = -8\left(\frac{G^4}{r^5}\;\frac{\vec{S}_1}{m_1}\cdot\vec{v}_2\times\vec{n}\,m_1^2\;m_2^3\right), \tag{A.47}$$

$$\text{Fig. 5(b4.2)} = -8\left(\frac{G^4}{r^5}\;\frac{\vec{S}_1}{m_1}\cdot\vec{v}_2\times\vec{n}\,m_1^2\;m_2^3\right), \tag{A.48}$$

$$\text{Fig. 5(b4.3)} = -8\left(\frac{G^4}{r^5}\;\frac{\vec{S}_1}{m_1}\cdot\vec{v}_2\times\vec{n}\,m_1^3\;m_2^2\right), \tag{A.49}$$

$$\text{Fig. 5(b4.4)} = -2\left(\frac{G^4}{r^5}\;\frac{\vec{S}_1}{m_1}\cdot\vec{v}_2\times\vec{n}\,m_1^3\;m_2^2\right), \tag{A.50}$$

$$\text{Fig. 5(b4.5)} = 8\left(\frac{G^4}{r^5}\;\frac{\vec{S}_1}{m_1}\cdot\vec{v}_1\times\vec{n}\,m_1^3\;m_2^2\right), \tag{A.51}$$

$$\text{Fig. 5(b4.6)} = 2\left(\frac{G^4}{r^5}\;\frac{\vec{S}_1}{m_1}\cdot\vec{v}_1\times\vec{n}\,m_1^3\;m_2^2\right), \tag{A.52}$$

$$\text{Fig. 5(b4.7)} = -\left(\frac{G^4}{r^5}\ \frac{\vec{S}_1}{m_1}\cdot\vec{v}_1\times\vec{n}\,m_1^2\ m_2^3\right), \tag{A.53}$$

$$\text{Fig. 5(b4.8)} = -8\left(\frac{G^4}{r^5}\ \frac{\vec{S}_1}{m_1}\cdot\vec{v}_1\times\vec{n}\,m_1^3\ m_2^2\right), \tag{A.54}$$

$$\text{Fig. 5(b4.9)} = 0, \tag{A.55}$$

$$\text{Fig. 5(b4.10)} = -\frac{1}{2}\ \left(\frac{G^4}{r^5}\frac{\vec{S}_1}{m_1}\cdot\ \vec{v}_1\times\vec{n}\,m_1^3 m_2^2\right), \tag{A.56}$$

$$\text{Fig. 5(b4.11)} = \left(\frac{G^4}{r^5}\frac{\vec{S}_1}{m_1}\cdot\ \vec{v}_2\times\vec{n}\,m_1^2 m_2^3\right), \tag{A.57}$$

$$\text{Fig. 5(b4.12)} = 2\left(\frac{G^4}{r^5}\frac{\vec{S}_1}{m_1}\cdot\ \vec{v}_1\times\vec{n}\,m_1^3 m_2^2\right), \tag{A.58}$$

$$\text{Fig. 5(b4.13)} = \frac{1}{2}\left(\frac{G^4}{r^5}\ \frac{\vec{S}_1}{m_1}\cdot\vec{v}_1\times\vec{n}\,m_1^3\ m_2^2\right) \tag{A.59}$$

$$\text{Fig. 6(b5.1)} = -64\left(\frac{G^4}{r^5}\ \frac{\vec{S}_1}{m_1}\cdot\vec{v}_2\times\vec{n}\,m_1 m_2^4\right), \tag{A.60}$$

$$\text{Fig. 6(b5.2)} = -\left(\frac{G^4}{r^5}\frac{\vec{S}_1}{m_1}\cdot\ \vec{v}_2\times\vec{n}\,m_1^4 m_2\right), \tag{A.61}$$

$$\text{Fig. 6(b5.3)} = \left(\frac{G^4}{r^5}\frac{\vec{S}_1}{m_1}\cdot\ \vec{v}_1\times\vec{n}\,m_1^4 m_2\right), \tag{A.62}$$

$$\text{Fig. 6(b5.4)} = 4\left(\frac{G^4}{r^5}\frac{\vec{S}_1}{m_1}\cdot\ \vec{v}_2\times\vec{n}\,m_1 m_2^4\right), \tag{A.63}$$

$$\text{Fig. 6(b5.5)} = -\frac{1}{4}\left(\frac{G^4}{r^5}\ \frac{\vec{S}_1}{m_1}\cdot\vec{v}_1\times\vec{n}\,m_1^4 m_2\right), \tag{A.64}$$

$$\text{Fig. 6(b5.6)} = 4\left(\frac{G^4}{r^5}\frac{\vec{S}_1}{m_1}\cdot\ \vec{v}_2\times\vec{n}\,m_1 m_2^4\right), \tag{A.65}$$

$$\text{Fig. 6(b5.7)} = \frac{1}{4}\left(\frac{G^4}{r^5}\ \frac{\vec{S}_1}{m_1}\cdot\vec{v}_1\times\vec{n}\,m_1^4 m_2\right), \tag{A.66}$$

$$\text{Fig. 6(b6.1)} = -4\left(\frac{G^4}{r^5}\frac{\vec{S}_1}{m_1}\cdot\ \vec{v}_2\times\vec{n}\,m_1^3 m_2^2\right), \tag{A.67}$$

$$\text{Fig. 6(b6.2)} = -4\left(\frac{G^4}{r^5}\frac{\vec{S}_1}{m_1}\cdot\ \vec{v}_2\times\vec{n}\,m_1^3 m_2^2\right), \tag{A.68}$$

$$\text{Fig. 6(b6.3)} = -\left(\frac{G^4}{r^5}\frac{\vec{S}_1}{m_1}\cdot\ \vec{v}_2\times\vec{n}\,m_1^2 m_2^3\right), \tag{A.69}$$

$$\text{Fig. 6(b6.4)} = -16\left(\frac{G^4}{r^5}\frac{\vec{S}_1}{m_1}\cdot\ \vec{v}_2\times\vec{n}\, m_1^2 m_2^3\right), \tag{A.70}$$

$$\text{Fig. 6(b6.5)} = \left(\frac{G^4}{r^5}\frac{\vec{S}_1}{m_1}\cdot\ \vec{v}_1\times\vec{n}\, m_1^2 m_2^3\right), \tag{A.71}$$

$$\text{Fig. 6(b6.6)} = 16\left(\frac{G^4}{r^5}\frac{\vec{S}_1}{m_1}\cdot\ \vec{v}_1\times\vec{n}\, m_1^2 m_2^3\right), \tag{A.72}$$

$$\text{Fig. 6(b6.7)} = -\frac{1}{2}\left(\frac{G^4}{r^5}\ \frac{\vec{S}_1}{m_1}\cdot\vec{v}_1\times\vec{n}\, m_1^3\ m_2^2\right), \tag{A.73}$$

$$\text{Fig. 6(b6.8)} = -\frac{1}{4}\left(\frac{G^4}{r^5}\ \frac{\vec{S}_1}{m_1}\cdot\vec{v}_1\times\vec{n}\, m_1^2\ m_2^3\right), \tag{A.74}$$

$$\text{Fig. 6(b6.9)} = 0, \tag{A.75}$$

$$\text{Fig. 6(b6.10)} = \frac{1}{2}\ \left(\frac{G^4}{r^5}\frac{\vec{S}_1}{m_1}\cdot\ \vec{v}_2\times\vec{n}\, m_1^3 m_2^2\right), \tag{A.76}$$

$$\text{Fig. 6(b6.11)} = 4\left(\frac{G^4}{r^5}\frac{\vec{S}_1}{m_1}\cdot\ \vec{v}_1\times\vec{n}\, m_1^2 m_2^3\right), \tag{A.77}$$

$$\text{Fig. 6(b6.12)} = \frac{1}{4}\left(\frac{G^4}{r^5}\ \frac{\vec{S}_1}{m_1}\cdot\vec{v}_1\times\vec{n}\, m_1^2\ m_2^3\right), \tag{A.78}$$

$$\text{Fig. 6(c1.1)} = 0, \tag{A.79}$$

$$\text{Fig. 6(c1.2)} = 0, \tag{A.80}$$

$$\text{Fig. 6(c1.3)} = 0, \tag{A.81}$$

$$\text{Fig. 6(c1.4)} = 0, \tag{A.82}$$

$$\text{Fig. 6(c1.5)} = 0, \tag{A.83}$$

$$\text{Fig. 6(c1.6)} = 0, \tag{A.84}$$

$$\text{Fig. 6(c1.7)} = 0, \tag{A.85}$$

$$\text{Fig. 6(c2.1)} = -64\left(\frac{G^4}{r^5}\frac{\vec{S}_1}{m_1}\cdot\ \vec{v}_2\times\vec{n}\, m_1 m_2^4\right), \tag{A.86}$$

$$\text{Fig. 6(c2.2)} = -\frac{16}{5}\left(\frac{G^4}{r^5}\ \frac{\vec{S}_1}{m_1}\cdot\vec{v}_2\times\vec{n}\, m_1^4 m_2\right), \tag{A.87}$$

$$\text{Fig. 6(c2.3)} = \frac{16}{5}\left(\frac{G^4}{r^5}\ \frac{\vec{S}_1}{m_1}\cdot\vec{v}_1\times\vec{n}\, m_1^4 m_2\right), \tag{A.88}$$

$$\text{Fig. 6(c3.1)} = -16\left(\frac{G^4}{r^5}\frac{\vec{S}_1}{m_1}\cdot\ \vec{v}_2\times\vec{n}\, m_1^2 m_2^3\right), \tag{A.89}$$

$$\text{Fig. 6(c3.2)} = -32\left(\frac{G^4}{r^5}\frac{\vec{S}_1}{m_1}\cdot\ \vec{v}_2\times\vec{n}\, m_1^2 m_2^3\right), \tag{A.90}$$

$$\text{Fig. 6(c3.3)} = -\frac{64}{5}\left(\frac{G^4}{r^5}\,\frac{\vec{S}_1}{m_1}\cdot\vec{v}_2\times\vec{n}\,m_1^3\,m_2^2\right), \tag{A.91}$$

$$\text{Fig. 6(c3.4)} = -\frac{32}{5}\left(\frac{G^4}{r^5}\,\frac{\vec{S}_1}{m_1}\cdot\vec{v}_2\times\vec{n}\,m_1^3\,m_2^2\right), \tag{A.92}$$

$$\text{Fig. 6(c3.5)} = \frac{64}{5}\left(\frac{G^4}{r^5}\,\frac{\vec{S}_1}{m_1}\cdot\vec{v}_1\times\vec{n}\,m_1^3\,m_2^2\right), \tag{A.93}$$

$$\text{Fig. 6(c3.6)} = \frac{16}{5}\left(\frac{G^4}{r^5}\,\frac{\vec{S}_1}{m_1}\cdot\vec{v}_1\times\vec{n}\,m_1^3\,m_2^2\right), \tag{A.94}$$

$$\text{Fig. 6(c3.7)} = \frac{16}{5}\left(\frac{G^4}{r^5}\,\frac{\vec{S}_1}{m_1}\cdot\vec{v}_1\times\vec{n}\,m_1^3\,m_2^2\right), \tag{A.95}$$

$$\begin{aligned}\text{Fig. 9(d1.1)} = {} & \frac{32}{3}\left(\frac{G^4}{r^5}\,\frac{\vec{S}_1}{m_1}\cdot\vec{v}_1\times\vec{n}\,m_1^2 m_2^3\,\left(\frac{1}{d-3}-4\ln\left(\frac{r}{R_0}\right)\right)\right) \\ & +\frac{112}{3}\left(\frac{G^4}{r^5}\frac{\vec{S}_1}{m_1}\cdot\ \vec{v}_1\times\vec{n}\,m_1^2 m_2^3\right),\end{aligned} \tag{A.96}$$

$$\begin{aligned}\text{Fig. 9(d1.2)} = {} & -\frac{32}{3}\left(\frac{G^4}{r^5}\,\frac{\vec{S}_1}{m_1}\cdot\vec{v}_2\times\vec{n}\,m_1^2 m_2^3\,\left(\frac{1}{d-3}-4\ln\left(\frac{r}{R_0}\right)\right)\right) \\ & -\frac{112}{3}\left(\frac{G^4}{r^5}\frac{\vec{S}_1}{m_1}\cdot\ \vec{v}_2\times\vec{n}\,m_1^2 m_2^3\right),\end{aligned} \tag{A.97}$$

$$\begin{aligned}\text{Fig. 9(d1.3)} = {} & \frac{128}{15}\left(\frac{G^4}{r^5}\,\frac{\vec{S}_1}{m_1}\cdot\vec{v}_1\times\vec{n}\,m_1^3 m_2^2\,\left(\frac{1}{d-3}-4\ln\left(\frac{r}{R_0}\right)\right)\right) \\ & +\frac{2176}{75}\left(\frac{G^4}{r^5}\frac{\vec{S}_1}{m_1}\cdot\ \vec{v}_1\times\vec{n}\,m_1^3 m_2^2\right),\end{aligned} \tag{A.98}$$

$$\begin{aligned}\text{Fig. 9(d1.4)} = {} & -\frac{128}{15}\left(\frac{G^4}{r^5}\,\frac{\vec{S}_1}{m_1}\cdot\vec{v}_2\times\vec{n}\,m_1^3 m_2^2\,\left(\frac{1}{d-3}-4\ln\left(\frac{r}{R_0}\right)\right)\right) \\ & -\frac{2176}{75}\left(\frac{G^4}{r^5}\frac{\vec{S}_1}{m_1}\cdot\ \vec{v}_2\times\vec{n}\,m_1^3 m_2^2\right),\end{aligned} \tag{A.99}$$

$$\text{Fig. 9(d2.1)} = -\frac{64}{3}\left(\frac{G^4}{r^5}\,\frac{\vec{S}_1}{m_1}\cdot\vec{v}_2\times\vec{n}\,m_1 m_2^4\right), \tag{A.100}$$

$$\text{Fig. 9(d2.2)} = \frac{32}{9}\left(\frac{G^4}{r^5}\,\frac{\vec{S}_1}{m_1}\cdot\vec{v}_1\times\vec{n}\,m_1^4 m_2\right), \tag{A.101}$$

$$\text{Fig. 9(d2.3)} = -\frac{32}{9}\left(\frac{G^4}{r^5}\,\frac{\vec{S}_1}{m_1}\cdot\vec{v}_2\times\vec{n}\,m_1^4 m_2\right), \tag{A.102}$$

$$\text{Fig. 6(e1.1)} = 0, \tag{A.103}$$

$$\text{Fig. 6(e1.2)} = 0, \tag{A.104}$$

$$\text{Fig. 6(e1.3)} = -\left(\frac{G^4}{r^5}\,\frac{\vec{S}_1}{m_1}\cdot\vec{v}_2\times\vec{n}\,m_1^2\;m_2^3\right), \tag{A.105}$$

$$\text{Fig. 6(e1.4)} = \frac{1}{4}\left(\frac{G^4}{r^5}\,\frac{\vec{S}_1}{m_1}\cdot\vec{v}_1\times\vec{n}\,m_1^2\;m_2^3\right), \tag{A.106}$$

$$\text{Fig. 6(e1.5)} = \frac{7}{4}\left(\frac{G^4}{r^5}\,\frac{\vec{S}_1}{m_1}\cdot\vec{v}_1\times\vec{n}\,m_1^2\;m_2^3\right) - 2\left(\frac{G^4}{r^5}\frac{\vec{S}_1}{m_1}\cdot\;\vec{v}_2\times\vec{n}\,m_1^2m_2^3\right), \tag{A.107}$$

$$\text{Fig. 6(e1.6)} = \left(\frac{G^4}{r^5}\frac{\vec{S}_1}{m_1}\cdot\;\vec{v}_1\times\vec{n}\,m_1^2m_2^3\right), \tag{A.108}$$

$$\text{Fig. 6(e2.1)} = -4\left(\frac{G^4}{r^5}\frac{\vec{S}_1}{m_1}\cdot\;\vec{v}_2\times\vec{n}\,m_1m_2^4\right), \tag{A.109}$$

$$\text{Fig. 6(e2.2)} = \frac{1}{4}\left(\frac{G^4}{r^5}\,\frac{\vec{S}_1}{m_1}\cdot\vec{v}_2\times\vec{n}\,m_1m_2^4\right), \tag{A.110}$$

$$\text{Fig. 6(e2.3)} = \frac{1}{8}\left(\frac{G^4}{r^5}\,\frac{\vec{S}_1}{m_1}\cdot\vec{v}_2\times\vec{n}\,m_1\;m_2^4\right) - \frac{3}{8}\left(\frac{G^4}{r^5}\,\frac{\vec{S}_1}{m_1}\cdot\vec{v}_1\times\vec{n}\,m_1m_2^4\right), \tag{A.111}$$

$$\text{Fig. 6(e3.1)} = 0, \tag{A.112}$$

$$\text{Fig. 6(e3.2)} = 0, \tag{A.113}$$

$$\text{Fig. 6(e3.3)} = 0, \tag{A.114}$$

$$\text{Fig. 6(e3.4)} = 8\left(\frac{G^4}{r^5}\frac{\vec{S}_1}{m_1}\cdot\;\vec{v}_2\times\vec{n}\,m_1^3m_2^2\right) - 8\left(\frac{G^4}{r^5}\,\frac{\vec{S}_1}{m_1}\cdot\vec{v}_1\times\vec{n}\,m_1^3\;m_2^2\right) \tag{A.115}$$

$$\text{Fig. 7(e4.1)} = 0, \tag{A.116}$$

$$\text{Fig. 7(e4.2)} = 0, \tag{A.117}$$

$$\text{Fig. 7(e4.3)} = 0, \tag{A.118}$$

$$\text{Fig. 7(e4.4)} = 0, \tag{A.119}$$

$$\text{Fig. 7(e4.5)} = 0, \tag{A.120}$$

$$\text{Fig. 7(e4.6)} = 0, \tag{A.121}$$

$$\text{Fig. 7(e4.7)} = 0, \tag{A.122}$$

$$\text{Fig. 7(e4.8)} = 0, \tag{A.123}$$

$$\text{Fig. 7(e4.9)} = 0, \tag{A.124}$$

$$\text{Fig. 7(e4.10)} = 0, \tag{A.125}$$

$$\text{Fig. 7(e4.11)} = 0, \tag{A.126}$$

$$\text{Fig. 7(e4.12)} = 0, \tag{A.127}$$

$$\text{Fig. 7(e4.13)} = 0, \tag{A.128}$$

$$\text{Fig. 7(e4.14)} = 0, \tag{A.129}$$

$$\text{Fig. 7(e4.15)} = 0, \tag{A.130}$$

$$\text{Fig. 7(e4.16)} = 0, \tag{A.131}$$

$$\text{Fig. 7(e4.17)} = 0, \tag{A.132}$$

$$\text{Fig. 7(e4.18)} = 0, \tag{A.133}$$

$$\text{Fig. 7(e5.1)} = 128 \left( \frac{G^4}{r^5} \frac{\vec{S}_1}{m_1} \cdot \ \vec{v}_2 \times \vec{n}\, m_1 m_2^4 \right), \tag{A.134}$$

$$\text{Fig. 7(e5.2)} = \frac{24}{5} \left( \frac{G^4}{r^5} \ \frac{\vec{S}_1}{m_1} \cdot \vec{v}_2 \times \vec{n}\, m_1^4 m_2 \right), \tag{A.135}$$

$$\text{Fig. 7(e5.3)} = -\frac{16}{5} \left( \frac{G^4}{r^5} \ \frac{\vec{S}_1}{m_1} \cdot \vec{v}_1 \times \vec{n}\, m_1^4 m_2 \right), \tag{A.136}$$

$$\text{Fig. 7(e5.4)} = -\frac{8}{5} \left( \frac{G^4}{r^5} \ \frac{\vec{S}_1}{m_1} \cdot \vec{v}_1 \times \vec{n}\, m_1^4 m_2 \right), \tag{A.137}$$

$$\text{Fig. 7(e5.5)} = -\frac{2}{3} \left( \frac{G^4}{r^5} \ \frac{\vec{S}_1}{m_1} \cdot \vec{v}_1 \times \vec{n}\, m_1^4 m_2 \right), \tag{A.138}$$

$$\text{Fig. 7(e5.6)} = \frac{8}{3} \left( \frac{G^4}{r^5} \ \frac{\vec{S}_1}{m_1} \cdot \vec{v}_2 \times \vec{n}\, m_1 m_2^4 \right), \tag{A.139}$$

$$\text{Fig. 7(e5.7)} = \frac{2}{3} \left( \frac{G^4}{r^5} \ \frac{\vec{S}_1}{m_1} \cdot \vec{v}_2 \times \vec{n}\, m_1^4 m_2 \right), \tag{A.140}$$

$$\text{Fig. 7(e5.8)} = -\frac{6}{5} \left( \frac{G^4}{r^5} \ \frac{\vec{S}_1}{m_1} \cdot \vec{v}_1 \times \vec{n}\, m_1^4 m_2 \right), \tag{A.141}$$

$$\text{Fig. 7(e5.9)} = -\frac{4}{5} \left( \frac{G^4}{r^5} \ \frac{\vec{S}_1}{m_1} \cdot \vec{v}_1 \times \vec{n}\, m_1^4 m_2 \right), \tag{A.142}$$

$$\text{Fig. 7(e5.10)} = \frac{8}{5} \left( \frac{G^4}{r^5} \ \frac{\vec{S}_1}{m_1} \cdot \vec{v}_2 \times \vec{n}\, m_1 m_2^4 \right), \tag{A.143}$$

$$\text{Fig. 7(e5.11)} = \frac{2}{5} \left( \frac{G^4}{r^5} \ \frac{\vec{S}_1}{m_1} \cdot \vec{v}_2 \times \vec{n}\, m_1^4 m_2 \right), \tag{A.144}$$

$$\text{Fig. 7(e5.12)} = 2 \left( \frac{G^4}{r^5} \frac{\vec{S}_1}{m_1} \cdot \ \vec{v}_1 \times \vec{n}\, m_1^4 m_2 \right), \tag{A.145}$$

$$\text{Fig. 7(e5.13)} = -8 \left( \frac{G^4}{r^5} \frac{\vec{S}_1}{m_1} \cdot \ \vec{v}_2 \times \vec{n}\, m_1 m_2^4 \right), \tag{A.146}$$

$$\text{Fig. 7(e5.14)} = \frac{1}{5} \left( \frac{G^4}{r^5} \ \frac{\vec{S}_1}{m_1} \cdot \vec{v}_1 \times \vec{n}\, m_1^4 m_2 \right), \tag{A.147}$$

$$\text{Fig. 7(e5.15)} = -\frac{1}{5} \left( \frac{G^4}{r^5} \ \frac{\vec{S}_1}{m_1} \cdot \vec{v}_1 \times \vec{n}\, m_1^4 m_2 \right), \tag{A.148}$$

$$\text{Fig. 7(e5.16)} = -\frac{8}{5} \left( \frac{G^4}{r^5} \ \frac{\vec{S}_1}{m_1} \cdot \vec{v}_2 \times \vec{n}\, m_1 m_2^4 \right), \tag{A.149}$$

$$\text{Fig. 7(e5.17)} = \frac{3}{5}\left(\frac{G^4}{r^5}\ \frac{\vec{S}_1}{m_1}\cdot\vec{v}_1\times\vec{n}\,m_1^4 m_2\right), \tag{A.150}$$

$$\text{Fig. 7(e5.18)} = -\left(\frac{G^4}{r^5}\frac{\vec{S}_1}{m_1}\cdot\ \vec{v}_1\times\vec{n}\,m_1^4 m_2\right), \tag{A.151}$$

$$\text{Fig. 7(e6.1)} = 32\left(\frac{G^4}{r^5}\frac{\vec{S}_1}{m_1}\cdot\ \vec{v}_2\times\vec{n}\,m_1^2 m_2^3\right), \tag{A.152}$$

$$\text{Fig. 7(e6.2)} = \frac{24}{5}\left(\frac{G^4}{r^5}\ \frac{\vec{S}_1}{m_1}\cdot\vec{v}_2\times\vec{n}\,m_1^3\ m_2^2\right), \tag{A.153}$$

$$\text{Fig. 7(e6.3)} = -\frac{64}{5}\left(\frac{G^4}{r^5}\ \frac{\vec{S}_1}{m_1}\cdot\vec{v}_1\times\vec{n}\,m_1^3\ m_2^2\right), \tag{A.154}$$

$$\text{Fig. 7(e6.4)} = -\frac{8}{5}\left(\frac{G^4}{r^5}\ \frac{\vec{S}_1}{m_1}\cdot\vec{v}_1\times\vec{n}\,m_1^3\ m_2^2\right), \tag{A.155}$$

$$\text{Fig. 7(e6.5)} = -\frac{2}{3}\left(\frac{G^4}{r^5}\ \frac{\vec{S}_1}{m_1}\cdot\vec{v}_1\times\vec{n}\,m_1^2\ m_2^3\right), \tag{A.156}$$

$$\text{Fig. 7(e6.6)} = \frac{8}{3}\left(\frac{G^4}{r^5}\ \frac{\vec{S}_1}{m_1}\cdot\vec{v}_2\times\vec{n}\,m_1^3\ m_2^2\right), \tag{A.157}$$

$$\text{Fig. 7(e6.7)} = \frac{2}{3}\left(\frac{G^4}{r^5}\ \frac{\vec{S}_1}{m_1}\cdot\vec{v}_2\times\vec{n}\,m_1^2\ m_2^3\right), \tag{A.158}$$

$$\text{Fig. 7(e6.8)} = -2\left(\frac{G^4}{r^5}\ \frac{\vec{S}_1}{m_1}\cdot\vec{v}_1\times\vec{n}\,m_1^2\ m_2^3\right), \tag{A.159}$$

$$\text{Fig. 7(e6.9)} = -\frac{4}{5}\left(\frac{G^4}{r^5}\ \frac{\vec{S}_1}{m_1}\cdot\vec{v}_1\times\vec{n}\,m_1^3\ m_2^2\right), \tag{A.160}$$

$$\text{Fig. 7(e6.10)} = \frac{2}{5}\left(\frac{G^4}{r^5}\ \frac{\vec{S}_1}{m_1}\cdot\vec{v}_2\times\vec{n}\,m_1^2\ m_2^3\right), \tag{A.161}$$

$$\text{Fig. 7(e6.11)} = \frac{8}{5}\left(\frac{G^4}{r^5}\ \frac{\vec{S}_1}{m_1}\cdot\vec{v}_2\times\vec{n}\,m_1^3\ m_2^2\right), \tag{A.162}$$

$$\text{Fig. 7(e6.12)} = 2\left(\frac{G^4}{r^5}\ \frac{\vec{S}_1}{m_1}\cdot\vec{v}_1\times\vec{n}\,m_1^3\ m_2^2\right), \tag{A.163}$$

$$\text{Fig. 7(e6.13)} = -2\left(\frac{G^4}{r^5}\ \frac{\vec{S}_1}{m_1}\cdot\vec{v}_2\times\vec{n}\,m_1^2\ m_2^3\right), \tag{A.164}$$

$$\text{Fig. 7(e6.14)} = \frac{4}{5}\left(\frac{G^4}{r^5}\ \frac{\vec{S}_1}{m_1}\cdot\vec{v}_1\times\vec{n}\,m_1^3\ m_2^2\right), \tag{A.165}$$

$$\text{Fig. 7(e6.15)} = -\frac{1}{5}\left(\frac{G^4}{r^5}\ \frac{\vec{S}_1}{m_1}\cdot\vec{v}_1\times\vec{n}\,m_1^3\ m_2^2\right), \tag{A.166}$$

$$\text{Fig. 7(e6.16)} = -\frac{2}{5}\left(\frac{G^4}{r^5}\,\frac{\vec{S}_1}{m_1}\cdot\vec{v}_2\times\vec{n}\,m_1^2\;m_2^3\right), \tag{A.167}$$

$$\text{Fig. 7(e6.17)} = \frac{12}{5}\left(\frac{G^4}{r^5}\,\frac{\vec{S}_1}{m_1}\cdot\vec{v}_1\times\vec{n}\,m_1^3\;m_2^2\right), \tag{A.168}$$

$$\text{Fig. 7(e6.18)} = -\left(\frac{G^4}{r^5}\,\frac{\vec{S}_1}{m_1}\cdot\vec{v}_1\times\vec{n}\,m_1^3\;m_2^2\right) \tag{A.169}$$

$$\text{Fig. 8(e7.1)} = 32\left(\frac{G^4}{r^5}\,\frac{\vec{S}_1}{m_1}\cdot\vec{v}_2\times\vec{n}\,m_1^2\;m_2^3\right), \tag{A.170}$$

$$\text{Fig. 8(e7.2)} = 32\left(\frac{G^4}{r^5}\,\frac{\vec{S}_1}{m_1}\cdot\vec{v}_2\times\vec{n}\,m_1^2\;m_2^3\right), \tag{A.171}$$

$$\text{Fig. 8(e7.3)} = \frac{96}{5}\left(\frac{G^4}{r^5}\,\frac{\vec{S}_1}{m_1}\cdot\vec{v}_2\times\vec{n}\,m_1^3\;m_2^2\right), \tag{A.172}$$

$$\text{Fig. 8(e7.4)} = \frac{24}{5}\left(\frac{G^4}{r^5}\,\frac{\vec{S}_1}{m_1}\cdot\vec{v}_2\times\vec{n}\,m_1^3\;m_2^2\right), \tag{A.173}$$

$$\text{Fig. 8(e7.5)} = -\frac{16}{5}\left(\frac{G^4}{r^5}\,\frac{\vec{S}_1}{m_1}\cdot\vec{v}_1\times\vec{n}\,m_1^3\;m_2^2\right), \tag{A.174}$$

$$\text{Fig. 8(e7.6)} = -\frac{16}{5}\left(\frac{G^4}{r^5}\,\frac{\vec{S}_1}{m_1}\cdot\vec{v}_1\times\vec{n}\,m_1^3\;m_2^2\right), \tag{A.175}$$

$$\text{Fig. 8(e7.7)} = -\frac{32}{5}\left(\frac{G^4}{r^5}\,\frac{\vec{S}_1}{m_1}\cdot\vec{v}_1\times\vec{n}\,m_1^3\;m_2^2\right), \tag{A.176}$$

$$\text{Fig. 8(e7.8)} = -\frac{8}{5}\left(\frac{G^4}{r^5}\,\frac{\vec{S}_1}{m_1}\cdot\vec{v}_1\times\vec{n}\,m_1^3\;m_2^2\right), \tag{A.177}$$

$$\text{Fig. 8(e7.9)} = -4\left(\frac{G^4}{r^5}\,\frac{\vec{S}_1}{m_1}\cdot\vec{v}_1\times\vec{n}\,m_1^2\;m_2^3\right), \tag{A.178}$$

$$\text{Fig. 8(e7.10)} = -\frac{12}{5}\left(\frac{G^4}{r^5}\,\frac{\vec{S}_1}{m_1}\cdot\vec{v}_1\times\vec{n}\,m_1^3\;m_2^2\right), \tag{A.179}$$

$$\text{Fig. 8(e7.11)} = -\frac{4}{5}\left(\frac{G^4}{r^5}\,\frac{\vec{S}_1}{m_1}\cdot\vec{v}_1\times\vec{n}\,m_1^3\;m_2^2\right), \tag{A.180}$$

$$\text{Fig. 8(e7.12)} = -\frac{4}{3}\left(\frac{G^4}{r^5}\,\frac{\vec{S}_1}{m_1}\cdot\vec{v}_1\times\vec{n}\,m_1^2\;m_2^3\right), \tag{A.181}$$

$$\text{Fig. 8(e7.13)} = \frac{16}{3}\left(\frac{G^4}{r^5}\,\frac{\vec{S}_1}{m_1}\cdot\vec{v}_2\times\vec{n}\,m_1^3\;m_2^2\right), \tag{A.182}$$

$$\text{Fig. 8(e7.14)} = \frac{4}{3}\left(\frac{G^4}{r^5}\,\frac{\vec{S}_1}{m_1}\cdot\vec{v}_2\times\vec{n}\,m_1^2\;m_2^3\right), \tag{A.183}$$

$$\text{Fig. 8(e7.15)} = \frac{4}{5}\left(\frac{G^4}{r^5}\,\frac{\vec{S}_1}{m_1}\cdot\vec{v}_2\times\vec{n}\,m_1^2\,m_2^3\right), \tag{A.184}$$

$$\text{Fig. 8(e7.16)} = \frac{4}{5}\left(\frac{G^4}{r^5}\,\frac{\vec{S}_1}{m_1}\cdot\vec{v}_2\times\vec{n}\,m_1^3\,m_2^2\right), \tag{A.185}$$

$$\text{Fig. 8(e7.17)} = 8\left(\frac{G^4}{r^5}\,\frac{\vec{S}_1}{m_1}\cdot\vec{v}_1\times\vec{n}\,m_1^3\,m_2^2\right), \tag{A.186}$$

$$\text{Fig. 8(e7.18)} = 2\left(\frac{G^4}{r^5}\,\frac{\vec{S}_1}{m_1}\cdot\vec{v}_1\times\vec{n}\,m_1^3\,m_2^2\right), \tag{A.187}$$

$$\text{Fig. 8(e7.19)} = -4\left(\frac{G^4}{r^5}\,\frac{\vec{S}_1}{m_1}\cdot\vec{v}_2\times\vec{n}\,m_1^2\,m_2^3\right), \tag{A.188}$$

$$\text{Fig. 8(e7.20)} = \frac{2}{5}\left(\frac{G^4}{r^5}\,\frac{\vec{S}_1}{m_1}\cdot\vec{v}_1\times\vec{n}\,m_1^3\,m_2^2\right), \tag{A.189}$$

$$\text{Fig. 8(e7.21)} = -\frac{4}{5}\left(\frac{G^4}{r^5}\,\frac{\vec{S}_1}{m_1}\cdot\vec{v}_1\times\vec{n}\,m_1^3\,m_2^2\right), \tag{A.190}$$

$$\text{Fig. 8(e7.22)} = -\frac{1}{5}\left(\frac{G^4}{r^5}\,\frac{\vec{S}_1}{m_1}\cdot\vec{v}_1\times\vec{n}\,m_1^3\,m_2^2\right), \tag{A.191}$$

$$\text{Fig. 8(e7.23)} = -\frac{4}{5}\left(\frac{G^4}{r^5}\,\frac{\vec{S}_1}{m_1}\cdot\vec{v}_2\times\vec{n}\,m_1^2\,m_2^3\right), \tag{A.192}$$

$$\text{Fig. 8(e7.24)} = \frac{6}{5}\left(\frac{G^4}{r^5}\,\frac{\vec{S}_1}{m_1}\cdot\vec{v}_1\times\vec{n}\,m_1^3\,m_2^2\right), \tag{A.193}$$

$$\text{Fig. 8(e7.25)} = -4\left(\frac{G^4}{r^5}\,\frac{\vec{S}_1}{m_1}\cdot\vec{v}_1\times\vec{n}\,m_1^3\,m_2^2\right), \tag{A.194}$$

$$\text{Fig. 8(e7.26)} = -\left(\frac{G^4}{r^5}\,\frac{\vec{S}_1}{m_1}\cdot\vec{v}_1\times\vec{n}\,m_1^3\,m_2^2\right), \tag{A.195}$$

$$\text{Fig. 8(e8.1)} = 16\left(\frac{G^4}{r^5}\,\frac{\vec{S}_1}{m_1}\cdot\vec{v}_2\times\vec{n}\,m_1^2\,m_2^3\right), \tag{A.196}$$

$$\text{Fig. 8(e8.2)} = 4\left(\frac{G^4}{r^5}\,\frac{\vec{S}_1}{m_1}\cdot\vec{v}_2\times\vec{n}\,m_1^2\,m_2^3\right), \tag{A.197}$$

$$\text{Fig. 8(e8.3)} = 4\left(\frac{G^4}{r^5}\,\frac{\vec{S}_1}{m_1}\cdot\vec{v}_2\times\vec{n}\,m_1^3\,m_2^2\right), \tag{A.198}$$

$$\text{Fig. 8(e8.4)} = 4\left(\frac{G^4}{r^5}\,\frac{\vec{S}_1}{m_1}\cdot\vec{v}_2\times\vec{n}\,m_1^3\,m_2^2\right), \tag{A.199}$$

$$\text{Fig. 8(e8.5)} = -16\left(\frac{G^4}{r^5}\,\frac{\vec{S}_1}{m_1}\cdot\vec{v}_1\times\vec{n}\,m_1^2\,m_2^3\right), \tag{A.200}$$

$$\text{Fig. 8(e8.6)} = -4\left(\frac{G^4}{r^5}\,\frac{\vec{S}_1}{m_1}\cdot\vec{v}_1\times\vec{n}\,m_1^2\;m_2^3\right), \tag{A.201}$$

$$\text{Fig. 8(e8.7)} = -4\left(\frac{G^4}{r^5}\,\frac{\vec{S}_1}{m_1}\cdot\vec{v}_1\times\vec{n}\,m_1^3\;m_2^2\right), \tag{A.202}$$

$$\text{Fig. 8(e8.8)} = -4\left(\frac{G^4}{r^5}\,\frac{\vec{S}_1}{m_1}\cdot\vec{v}_1\times\vec{n}\,m_1^3\;m_2^2\right), \tag{A.203}$$

$$\text{Fig. 8(e8.9)} = -8\left(\frac{G^4}{r^5}\,\frac{\vec{S}_1}{m_1}\cdot\vec{v}_1\times\vec{n}\,m_1^3\;m_2^2\right), \tag{A.204}$$

$$\text{Fig. 8(e8.10)} = 32\left(\frac{G^4}{r^5}\,\frac{\vec{S}_1}{m_1}\cdot\vec{v}_2\times\vec{n}\,m_1^2\;m_2^3\right), \tag{A.205}$$

$$\text{Fig. 8(e8.11)} = 8\left(\frac{G^4}{r^5}\,\frac{\vec{S}_1}{m_1}\cdot\vec{v}_2\times\vec{n}\,m_1^3\;m_2^2\right), \tag{A.206}$$

$$\text{Fig. 8(e8.12)} = -12\left(\frac{G^4}{r^5}\,\frac{\vec{S}_1}{m_1}\cdot\vec{v}_1\times\vec{n}\,m_1^2\;m_2^3\right), \tag{A.207}$$

$$\text{Fig. 8(e8.13)} = -12\left(\frac{G^4}{r^5}\,\frac{\vec{S}_1}{m_1}\cdot\vec{v}_1\times\vec{n}\,m_1^3\;m_2^2\right), \tag{A.208}$$

$$\text{Fig. 8(e8.14)} = -12\left(\frac{G^4}{r^5}\,\frac{\vec{S}_1}{m_1}\cdot\vec{v}_1\times\vec{n}\,m_1^3\;m_2^2\right), \tag{A.209}$$

$$\text{Fig. 8(e8.15)} = 64\left(\frac{G^4}{r^5}\,\frac{\vec{S}_1}{m_1}\cdot\vec{v}_2\times\vec{n}\,m_1^2\;m_2^3\right), \tag{A.210}$$

$$\text{Fig. 8(e8.16)} = 16\left(\frac{G^4}{r^5}\,\frac{\vec{S}_1}{m_1}\cdot\vec{v}_2\times\vec{n}\,m_1^2\;m_2^3\right), \tag{A.211}$$

$$\text{Fig. 8(e8.17)} = 16\left(\frac{G^4}{r^5}\,\frac{\vec{S}_1}{m_1}\cdot\vec{v}_2\times\vec{n}\,m_1^3\;m_2^2\right), \tag{A.212}$$

$$\text{Fig. 8(e8.18)} = 16\left(\frac{G^4}{r^5}\,\frac{\vec{S}_1}{m_1}\cdot\vec{v}_2\times\vec{n}\,m_1^3\;m_2^2\right), \tag{A.213}$$

$$\text{Fig. 8(e8.19)} = 8\left(\frac{G^4}{r^5}\,\frac{\vec{S}_1}{m_1}\cdot\vec{v}_2\times\vec{n}\,m_1^2\;m_2^3\right) - 8\left(\frac{G^4}{r^5}\frac{\vec{S}_1}{m_1}\cdot\;\vec{v}_1\times\vec{n}\,m_1^2m_2^3\right), \tag{A.214}$$

$$\text{Fig. 8(e8.20)} = 2\left(\frac{G^4}{r^5}\frac{\vec{S}_1}{m_1}\cdot\;\vec{v}_2\times\vec{n}\,m_1^2m_2^3\right) - 2\left(\frac{G^4}{r^5}\,\frac{\vec{S}_1}{m_1}\cdot\vec{v}_1\times\vec{n}\,m_1^2\;m_2^3\right), \tag{A.215}$$

$$\text{Fig. 8(e8.21)} = 2\left(\frac{G^4}{r^5}\,\frac{\vec{S}_1}{m_1}\cdot\vec{v}_2\times\vec{n}\,m_1^3\;m_2^2\right) - 2\left(\frac{G^4}{r^5}\frac{\vec{S}_1}{m_1}\cdot\;\vec{v}_1\times\vec{n}\,m_1^3m_2^2\right), \tag{A.216}$$

$$\text{Fig. 8(e8.22)} = 2\left(\frac{G^4}{r^5}\frac{\vec{S}_1}{m_1}\cdot\;\vec{v}_2\times\vec{n}\,m_1^3m_2^2\right) - 2\left(\frac{G^4}{r^5}\,\frac{\vec{S}_1}{m_1}\cdot\vec{v}_1\times\vec{n}\,m_1^3\;m_2^2\right), \tag{A.217}$$

$$\text{Fig. 8(e8.23)} = 48\left(\frac{G^4}{r^5}\ \frac{\vec{S}_1}{m_1}\cdot\vec{v}_1\times\vec{n}\,m_1^2\ m_2^3\right) - 40\left(\frac{G^4}{r^5}\frac{\vec{S}_1}{m_1}\cdot\ \vec{v}_2\times\vec{n}\,m_1^2 m_2^3\right), \tag{A.218}$$

$$\text{Fig. 8(e8.24)} = 12\left(\frac{G^4}{r^5}\frac{\vec{S}_1}{m_1}\cdot\ \vec{v}_1\times\vec{n}\,m_1^2 m_2^3\right) - 10\left(\frac{G^4}{r^5}\ \frac{\vec{S}_1}{m_1}\cdot\vec{v}_2\times\vec{n}\,m_1^2\ m_2^3\right), \tag{A.219}$$

$$\text{Fig. 8(e8.25)} = 12\left(\frac{G^4}{r^5}\ \frac{\vec{S}_1}{m_1}\cdot\vec{v}_1\times\vec{n}\,m_1^3\ m_2^2\right) - 10\left(\frac{G^4}{r^5}\frac{\vec{S}_1}{m_1}\cdot\ \vec{v}_2\times\vec{n}\,m_1^3 m_2^2\right), \tag{A.220}$$

$$\text{Fig. 8(e8.26)} = 12\left(\frac{G^4}{r^5}\frac{\vec{S}_1}{m_1}\cdot\ \vec{v}_1\times\vec{n}\,m_1^3 m_2^2\right) - 10\left(\frac{G^4}{r^5}\ \frac{\vec{S}_1}{m_1}\cdot\vec{v}_2\times\vec{n}\,m_1^3\ m_2^2\right) \tag{A.221}$$

$$\begin{aligned}\text{Fig. 9(f1.1)} = \frac{64}{3}&\left(\frac{G^4}{r^5}\ \frac{\vec{S}_1}{m_1}\cdot\vec{v}_2\times\vec{n}\,m_1^2 m_2^3\ \left(\frac{1}{d-3} - 4\ln\left(\frac{r}{R_0}\right)\right)\right)\\ &+ \frac{224}{3}\left(\frac{G^4}{r^5}\frac{\vec{S}_1}{m_1}\cdot\ \vec{v}_2\times\vec{n}\,m_1^2 m_2^3\right),\end{aligned} \tag{A.222}$$

$$\begin{aligned}\text{Fig. 9(f1.2)} = -\frac{4}{3}&\left(\frac{G^4}{r^5}\ \frac{\vec{S}_1}{m_1}\cdot\vec{v}_2\times\vec{n}\,m_1^2 m_2^3\ \left(\frac{1}{d-3} - 4\ln\left(\frac{r}{R_0}\right)\right)\right)\\ &- \frac{14}{3}\left(\frac{G^4}{r^5}\frac{\vec{S}_1}{m_1}\cdot\ \vec{v}_2\times\vec{n}\,m_1^2 m_2^3\right),\end{aligned} \tag{A.223}$$

$$\begin{aligned}\text{Fig. 9(f1.3)} = -\frac{128}{15}&\left(\frac{G^4}{r^5}\ \frac{\vec{S}_1}{m_1}\cdot\vec{v}_1\times\vec{n}\,m_1^3 m_2^2\ \left(\frac{1}{d-3} - 4\ln\left(\frac{r}{R_0}\right)\right)\right)\\ &- \frac{2176}{75}\left(\frac{G^4}{r^5}\frac{\vec{S}_1}{m_1}\cdot\ \vec{v}_1\times\vec{n}\,m_1^3 m_2^2\right),\end{aligned} \tag{A.224}$$

$$\begin{aligned}\text{Fig. 9(f1.4)} = \frac{8}{15}&\left(\frac{G^4}{r^5}\ \frac{\vec{S}_1}{m_1}\cdot\vec{v}_1\times\vec{n}\,m_1^3 m_2^2\ \left(\frac{1}{d-3} - 4\ln\left(\frac{r}{R_0}\right)\right)\right)\\ &+ \frac{136}{75}\left(\frac{G^4}{r^5}\frac{\vec{S}_1}{m_1}\cdot\ \vec{v}_1\times\vec{n}\,m_1^3 m_2^2\right),\end{aligned} \tag{A.225}$$

$$\begin{aligned}\text{Fig. 9(f1.5)} = -\frac{64}{15}&\left(\frac{G^4}{r^5}\ \frac{\vec{S}_1}{m_1}\cdot\vec{v}_1\times\vec{n}\,m_1^3 m_2^2\ \left(\frac{1}{d-3} - 4\ln\left(\frac{r}{R_0}\right)\right)\right)\\ &- \frac{416}{25}\left(\frac{G^4}{r^5}\frac{\vec{S}_1}{m_1}\cdot\ \vec{v}_1\times\vec{n}\,m_1^3 m_2^2\right),\end{aligned} \tag{A.226}$$

$$\begin{aligned}\text{Fig. 9(f1.6)} = \frac{64}{5}&\left(\frac{G^4}{r^5}\ \frac{\vec{S}_1}{m_1}\cdot\vec{v}_2\times\vec{n}\,m_1^3 m_2^2\ \left(\frac{1}{d-3} - 4\ln\left(\frac{r}{R_0}\right)\right)\right)\\ &+ \frac{3424}{75}\left(\frac{G^4}{r^5}\frac{\vec{S}_1}{m_1}\cdot\ \vec{v}_2\times\vec{n}\,m_1^3 m_2^2\right),\end{aligned} \tag{A.227}$$

$$\text{Fig. 9(f1.7)} = \frac{16}{15}\left(\frac{G^4}{r^5}\ \frac{\vec{S}_1}{m_1}\cdot\vec{v}_2\times\vec{n}\,m_1^3 m_2^2\ \left(\frac{1}{d-3} - 4\ln\left(\frac{r}{R_0}\right)\right)\right) \tag{A.228}$$

$$+\frac{184}{25}\left(\frac{G^4}{r^5}\frac{\vec{S}_1}{m_1}\cdot\ \vec{v}_2\times\vec{n}\,m_1^3m_2^2\right),$$

$$\text{Fig. 9(f1.8)}=\frac{4}{3}\left(\frac{G^4}{r^5}\ \frac{\vec{S}_1}{m_1}\cdot\vec{v}_1\times\vec{n}\,m_1^2m_2^3\ \left(\frac{1}{d-3}-4\ln\left(\frac{r}{R_0}\right)\right)\right) \tag{A.229}$$

$$+\frac{16}{3}\left(\frac{G^4}{r^5}\frac{\vec{S}_1}{m_1}\cdot\ \vec{v}_1\times\vec{n}\,m_1^2m_2^3\right),$$

$$\text{Fig. 9(f1.9)}=\frac{4}{5}\left(\frac{G^4}{r^5}\ \frac{\vec{S}_1}{m_1}\cdot\vec{v}_2\times\vec{n}\,m_1^2m_2^3\ \left(\frac{1}{d-3}-4\ln\left(\frac{r}{R_0}\right)\right)\right) \tag{A.230}$$

$$+\frac{464}{75}\left(\frac{G^4}{r^5}\frac{\vec{S}_1}{m_1}\cdot\ \vec{v}_2\times\vec{n}\,m_1^2m_2^3\right),$$

$$\text{Fig. 9(f1.10)}=-\frac{4}{15}\left(\frac{G^4}{r^5}\ \frac{\vec{S}_1}{m_1}\cdot\vec{v}_1\times\vec{n}\,m_1^3m_2^2\ \left(\frac{1}{d-3}-4\ln\left(\frac{r}{R_0}\right)\right)\right) \tag{A.231}$$

$$-\frac{57}{50}\left(\frac{G^4}{r^5}\frac{\vec{S}_1}{m_1}\cdot\ \vec{v}_1\times\vec{n}\,m_1^3m_2^2\right),$$

$$\text{Fig. 9(f1.11)}=\frac{3}{5}\left(\frac{G^4}{r^5}\ \frac{\vec{S}_1}{m_1}\cdot\vec{v}_1\times\vec{n}\,m_1^2m_2^3\ \left(\frac{1}{d-3}-4\ln\left(\frac{r}{R_0}\right)\right)\right) \tag{A.232}$$

$$+\frac{187}{50}\left(\frac{G^4}{r^5}\frac{\vec{S}_1}{m_1}\cdot\ \vec{v}_1\times\vec{n}\,m_1^2m_2^3\right),$$

$$\text{Fig. 9(f1.12)}=\frac{1}{6}\left(\frac{G^4}{r^5}\ \frac{\vec{S}_1}{m_1}\cdot\vec{v}_2\times\vec{n}\,m_1^3\ m_2^2\right), \tag{A.233}$$

$$\text{Fig. 9(f1.13)}=-\frac{1}{3}\left(\frac{G^4}{r^5}\ \frac{\vec{S}_1}{m_1}\cdot\vec{v}_1\times\vec{n}\,m_1^2m_2^3\ \left(\frac{1}{d-3}-4\ln\left(\frac{r}{R_0}\right)\right)\right) \tag{A.234}$$

$$-\frac{11}{6}\left(\frac{G^4}{r^5}\frac{\vec{S}_1}{m_1}\cdot\ \vec{v}_1\times\vec{n}\,m_1^2m_2^3\right)$$

$$+\frac{1}{15}\ \left(\frac{G^4}{r^5}\frac{\vec{S}_1}{m_1}\cdot\ \vec{v}_2\times\vec{n}\,m_1^2m_2^3\ \left(\frac{1}{d-3}-4\ln\left(\frac{r}{R_0}\right)\right)\right)$$

$$+\frac{32}{75}\left(\frac{G^4}{r^5}\frac{\vec{S}_1}{m_1}\cdot\ \vec{v}_2\times\vec{n}\,m_1^2m_2^3\right),$$

$$\text{Fig. 9(f2.1)}=\frac{32}{3}\left(\frac{G^4}{r^5}\ \frac{\vec{S}_1}{m_1}\cdot\vec{v}_2\times\vec{n}\,m_1^2m_2^3\ \left(\frac{1}{d-3}-4\ln\left(\frac{r}{R_0}\right)\right)\right) \tag{A.235}$$

$$+\frac{112}{3}\left(\frac{G^4}{r^5}\frac{\vec{S}_1}{m_1}\cdot\ \vec{v}_2\times\vec{n}\,m_1^2m_2^3\right),$$

$$\text{Fig. 9(f2.2)}=\frac{128}{15}\left(\frac{G^4}{r^5}\ \frac{\vec{S}_1}{m_1}\cdot\vec{v}_2\times\vec{n}\,m_1^3m_2^2\ \left(\frac{1}{d-3}-4\ln\left(\frac{r}{R_0}\right)\right)\right) \tag{A.236}$$

$$+\frac{2176}{75}\left(\frac{G^4}{r^5}\frac{\vec{S}_1}{m_1}\cdot\ \vec{v}_2\times\vec{n}\,m_1^3m_2^2\right),$$

$$\text{Fig. 9(f2.3)}=-\frac{8}{15}\left(\frac{G^4}{r^5}\ \frac{\vec{S}_1}{m_1}\cdot\vec{v}_2\times\vec{n}\,m_1^3m_2^2\ \left(\frac{1}{d-3}-4\ln\left(\frac{r}{R_0}\right)\right)\right) \tag{A.237}$$

$$-\frac{136}{75}\left(\frac{G^4}{r^5}\frac{\vec{S}_1}{m_1}\cdot\ \vec{v}_2\times\vec{n}\,m_1^3m_2^2\right),$$

$$\text{Fig. 9(f2.4)}=\frac{8}{105}\left(\frac{G^4}{r^5}\ \frac{\vec{S}_1}{m_1}\cdot\vec{v}_1\times\vec{n}\,m_1^3m_2^2\ \left(\frac{1}{d-3}-4\ln\left(\frac{r}{R_0}\right)\right)\right) \tag{A.238}$$

$$+\frac{272}{3675}\left(\frac{G^4}{r^5}\frac{\vec{S}_1}{m_1}\cdot\ \vec{v}_1\times\vec{n}\,m_1^3m_2^2\right),$$

$$\text{Fig. 9(f2.5)}=\frac{1}{21}\left(\frac{G^4}{r^5}\ \frac{\vec{S}_1}{m_1}\cdot\vec{v}_1\times\vec{n}\,m_1^3m_2^2\ \left(\frac{1}{d-3}-4\ln\left(\frac{r}{R_0}\right)\right)\right) \tag{A.239}$$

$$+\frac{19}{98}\left(\frac{G^4}{r^5}\frac{\vec{S}_1}{m_1}\cdot\ \vec{v}_1\times\vec{n}\,m_1^3m_2^2\right),$$

$$\text{Fig. 9(f2.6)}=-\frac{2}{105}\left(\frac{G^4}{r^5}\ \frac{\vec{S}_1}{m_1}\cdot\vec{v}_1\times\vec{n}\,m_1^3m_2^2\ \left(\frac{1}{d-3}-4\ln\left(\frac{r}{R_0}\right)\right)\right) \tag{A.240}$$

$$-\frac{313}{3675}\left(\frac{G^4}{r^5}\frac{\vec{S}_1}{m_1}\cdot\ \vec{v}_1\times\vec{n}\,m_1^3m_2^2\right),$$

$$\text{Fig. 9(f3.1)}=64\left(\frac{G^4}{r^5}\frac{\vec{S}_1}{m_1}\cdot\ \vec{v}_2\times\vec{n}\,m_1m_2^4\right), \tag{A.241}$$

$$\text{Fig. 9(f3.2)}=-4\left(\frac{G^4}{r^5}\frac{\vec{S}_1}{m_1}\cdot\ \vec{v}_2\times\vec{n}\,m_1m_2^4\right), \tag{A.242}$$

$$\text{Fig. 9(f3.3)}=-\frac{64}{9}\left(\frac{G^4}{r^5}\ \frac{\vec{S}_1}{m_1}\cdot\vec{v}_1\times\vec{n}\,m_1^4m_2\right), \tag{A.243}$$

$$\text{Fig. 9(f3.4)}=\frac{4}{9}\left(\frac{G^4}{r^5}\ \frac{\vec{S}_1}{m_1}\cdot\vec{v}_1\times\vec{n}\,m_1^4m_2\right), \tag{A.244}$$

$$\text{Fig. 9(f3.5)}=-\frac{32}{9}\left(\frac{G^4}{r^5}\ \frac{\vec{S}_1}{m_1}\cdot\vec{v}_1\times\vec{n}\,m_1^4m_2\right), \tag{A.245}$$

$$\text{Fig. 9(f3.6)}=\frac{64}{9}\left(\frac{G^4}{r^5}\ \frac{\vec{S}_1}{m_1}\cdot\vec{v}_2\times\vec{n}\,m_1^4m_2\right), \tag{A.246}$$

$$\text{Fig. 9(f3.7)}=\frac{8}{9}\left(\frac{G^4}{r^5}\ \frac{\vec{S}_1}{m_1}\cdot\vec{v}_2\times\vec{n}\,m_1^4m_2\right), \tag{A.247}$$

$$\text{Fig. 9(f3.8)}=\frac{4}{3}\left(\frac{G^4}{r^5}\ \frac{\vec{S}_1}{m_1}\cdot\vec{v}_2\times\vec{n}\,m_1m_2^4\right), \tag{A.248}$$

$$\text{Fig. 9(f3.9)}=0, \tag{A.249}$$

$$\text{Fig. 9(f3.10)} = \frac{4}{9}\left(\frac{G^4}{r^5}\,\frac{\vec{S}_1}{m_1}\cdot\vec{v}_1\times\vec{n}\,m_1^4m_2\right), \tag{A.250}$$

$$\text{Fig. 9(f3.11)} = -\frac{5}{18}\left(\frac{G^4}{r^5}\,\frac{\vec{S}_1}{m_1}\cdot\vec{v}_1\times\vec{n}\,m_1m_2^4\right), \tag{A.251}$$

$$\text{Fig. 9(f3.12)} = 0, \tag{A.252}$$

$$\text{Fig. 9(f3.13)} = -\frac{1}{9}\left(\frac{G^4}{r^5}\,\frac{\vec{S}_1}{m_1}\cdot\vec{v}_2\times\vec{n}\,m_1m_2^4\right), \tag{A.253}$$

$$\text{Fig. 9(f4.1)} = 64\left(\frac{G^4}{r^5}\frac{\vec{S}_1}{m_1}\cdot\ \vec{v}_2\times\vec{n}\,m_1m_2^4\right), \tag{A.254}$$

$$\text{Fig. 9(f4.2)} = -\frac{32}{9}\left(\frac{G^4}{r^5}\,\frac{\vec{S}_1}{m_1}\cdot\vec{v}_1\times\vec{n}\,m_1^4m_2\right), \tag{A.255}$$

$$\text{Fig. 9(f4.3)} = -\frac{32}{15}\left(\frac{G^4}{r^5}\,\frac{\vec{S}_1}{m_1}\cdot\vec{v}_1\times\vec{n}\,m_1^4m_2\right), \tag{A.256}$$

$$\text{Fig. 9(f4.4)} = \frac{416}{45}\left(\frac{G^4}{r^5}\,\frac{\vec{S}_1}{m_1}\cdot\vec{v}_2\times\vec{n}\,m_1^4m_2\right), \tag{A.257}$$

$$\text{Fig. 9(f4.5)} = -\frac{8}{45}\left(\frac{G^4}{r^5}\,\frac{\vec{S}_1}{m_1}\cdot\vec{v}_1\times\vec{n}\,m_1^4m_2\right), \tag{A.258}$$

$$\begin{aligned}\text{Fig. 9(f4.6)} = &-\frac{32}{35}\left(\frac{G^4}{r^5}\,\frac{\vec{S}_1}{m_1}\cdot\vec{v}_1\times\vec{n}\,m_1^4m_2\ \left(\frac{1}{d-3}-4\ln\left(\frac{r}{R_0}\right)\right)\right)\\ &-\frac{14552}{11025}\left(\frac{G^4}{r^5}\frac{\vec{S}_1}{m_1}\cdot\ \vec{v}_1\times\vec{n}\,m_1^4m_2\right),\end{aligned} \tag{A.259}$$

$$\begin{aligned}\text{Fig. 9(f4.7)} = &-\frac{4}{105}\left(\frac{G^4}{r^5}\,\frac{\vec{S}_1}{m_1}\cdot\vec{v}_1\times\vec{n}\,m_1^4m_2\ \left(\frac{1}{d-3}-4\ln\left(\frac{r}{R_0}\right)\right)\right)\\ &-\frac{2753}{11025}\left(\frac{G^4}{r^5}\frac{\vec{S}_1}{m_1}\cdot\ \vec{v}_1\times\vec{n}\,m_1^4m_2\right),\end{aligned} \tag{A.260}$$

$$\begin{aligned}\text{Fig. 9(f4.8)} = &-\frac{4}{105}\left(\frac{G^4}{r^5}\,\frac{\vec{S}_1}{m_1}\cdot\vec{v}_1\times\vec{n}\,m_1^4m_2\ \left(\frac{1}{d-3}-4\ln\left(\frac{r}{R_0}\right)\right)\right)\\ &-\frac{478}{11025}\left(\frac{G^4}{r^5}\frac{\vec{S}_1}{m_1}\cdot\ \vec{v}_1\times\vec{n}\,m_1^4m_2\right),\end{aligned} \tag{A.261}$$

$$\begin{aligned}\text{Fig. 9(f5.1)} = &-\frac{64}{3}\left(\frac{G^4}{r^5}\,\frac{\vec{S}_1}{m_1}\cdot\vec{v}_1\times\vec{n}\,m_1^2m_2^3\ \left(\frac{1}{d-3}-4\ln\left(\frac{r}{R_0}\right)\right)\right)\\ &-\frac{224}{3}\left(\frac{G^4}{r^5}\frac{\vec{S}_1}{m_1}\cdot\ \vec{v}_1\times\vec{n}\,m_1^2m_2^3\right),\end{aligned} \tag{A.262}$$

$$\text{Fig. 9(f5.2)} = 0, \tag{A.263}$$

$$\text{Fig. 9(f5.3)} = -\frac{64}{3}\left(\frac{G^4}{r^5}\ \frac{\vec{S}_1}{m_1}\cdot\vec{v}_1\times\vec{n}\,m_1^2m_2^3\ \left(\frac{1}{d-3}-4\ln\left(\frac{r}{R_0}\right)\right)\right) \tag{A.264}$$
$$-\ 64\ \left(\frac{G^4}{r^5}\frac{\vec{S}_1}{m_1}\cdot\ \vec{v}_1\times\vec{n}\,m_1^2m_2^3\right),$$

$$\text{Fig. 9(f5.4)} = \frac{64}{15}\left(\frac{G^4}{r^5}\ \frac{\vec{S}_1}{m_1}\cdot\vec{v}_2\times\vec{n}\,m_1^3m_2^2\ \left(\frac{1}{d-3}-4\ln\left(\frac{r}{R_0}\right)\right)\right) \tag{A.265}$$
$$+\ \frac{256}{25}\left(\frac{G^4}{r^5}\frac{\vec{S}_1}{m_1}\cdot\ \vec{v}_2\times\vec{n}\,m_1^3m_2^2\right),$$

$$\text{Fig. 9(f5.5)} = -4\left(\frac{G^4}{r^5}\frac{\vec{S}_1}{m_1}\cdot\ \vec{v}_1\times\vec{n}\,m_1^2m_2^3\right) \tag{A.266}$$
$$-\ \frac{8}{3}\ \left(\frac{G^4}{r^5}\frac{\vec{S}_1}{m_1}\cdot\ \vec{v}_2\times\vec{n}\,m_1^2m_2^3\ \left(\frac{1}{d-3}-4\ln\left(\frac{r}{R_0}\right)\right)\right)$$
$$-\ \frac{20}{3}\left(\frac{G^4}{r^5}\frac{\vec{S}_1}{m_1}\cdot\ \vec{v}_2\times\vec{n}\,m_1^2m_2^3\right),$$

$$\text{Fig. 9(f5.6)} = -\frac{176}{15}\left(\frac{G^4}{r^5}\ \frac{\vec{S}_1}{m_1}\cdot\vec{v}_1\times\vec{n}\,m_1^3m_2^2\ \left(\frac{1}{d-3}-4\ln\left(\frac{r}{R_0}\right)\right)\right) \tag{A.267}$$
$$-\ \frac{2392}{75}\left(\frac{G^4}{r^5}\frac{\vec{S}_1}{m_1}\cdot\ \vec{v}_1\times\vec{n}\,m_1^3m_2^2\right),$$

$$\text{Fig. 9(f5.7)} = -\frac{64}{5}\left(\frac{G^4}{r^5}\ \frac{\vec{S}_1}{m_1}\cdot\vec{v}_1\times\vec{n}\,m_1^3m_2^2\ \left(\frac{1}{d-3}-4\ln\left(\frac{r}{R_0}\right)\right)\right) \tag{A.268}$$
$$-\ \frac{2944}{75}\left(\frac{G^4}{r^5}\frac{\vec{S}_1}{m_1}\cdot\ \vec{v}_1\times\vec{n}\,m_1^3m_2^2\right),$$

$$\text{Fig. 9(f5.8)} = \frac{176}{15}\left(\frac{G^4}{r^5}\ \frac{\vec{S}_1}{m_1}\cdot\vec{v}_2\times\vec{n}\,m_1^3m_2^2\ \left(\frac{1}{d-3}-4\ln\left(\frac{r}{R_0}\right)\right)\right) \tag{A.269}$$
$$+\ \frac{2392}{75}\left(\frac{G^4}{r^5}\frac{\vec{S}_1}{m_1}\cdot\ \vec{v}_2\times\vec{n}\,m_1^3m_2^2\right),$$

$$\text{Fig. 9(f5.9)} = \frac{32}{3}\left(\frac{G^4}{r^5}\ \frac{\vec{S}_1}{m_1}\cdot\vec{v}_2\times\vec{n}\,m_1^2m_2^3\ \left(\frac{1}{d-3}-4\ln\left(\frac{r}{R_0}\right)\right)\right) \tag{A.270}$$
$$+\ \frac{80}{3}\left(\frac{G^4}{r^5}\frac{\vec{S}_1}{m_1}\cdot\ \vec{v}_2\times\vec{n}\,m_1^2m_2^3\right),$$

$$\text{Fig. 9(f5.10)} = \frac{4}{15}\left(\frac{G^4}{r^5}\ \frac{\vec{S}_1}{m_1}\cdot\vec{v}_1\times\vec{n}\,m_1^3m_2^2\ \left(\frac{1}{d-3}-4\ln\left(\frac{r}{R_0}\right)\right)\right) \tag{A.271}$$
$$+\ \frac{88}{75}\left(\frac{G^4}{r^5}\frac{\vec{S}_1}{m_1}\cdot\ \vec{v}_1\times\vec{n}\,m_1^3m_2^2\right)$$

$$
\begin{aligned}
& - \frac{8}{3} \left( \frac{G^4}{r^5} \frac{\vec{S}_1}{m_1} \cdot \; \vec{v}_2 \times \vec{n} \, m_1^3 m_2^2 \; \left( \frac{1}{d-3} - 4 \ln \left( \frac{r}{R_0} \right) \right) \right) \\
& - \frac{20}{3} \left( \frac{G^4}{r^5} \frac{\vec{S}_1}{m_1} \cdot \; \vec{v}_2 \times \vec{n} \, m_1^3 m_2^2 \right),
\end{aligned}
$$

$$
\begin{aligned}
\text{Fig. 9(f5.11)} = & \left( \frac{2}{3} \left( -80 + 9\pi^2 \right) \right) \left( \frac{G^4}{r^5} \frac{\vec{S}_1}{m_1} \cdot \; \vec{v}_2 \times \vec{n} \, m_1^3 m_2^2 \right) \\
& - \frac{52}{3} \left( \frac{G^4}{r^5} \frac{\vec{S}_1}{m_1} \cdot \; \vec{v}_2 \times \vec{n} \, m_1^3 m_2^2 \; \left( \frac{1}{d-3} - 4 \ln \left( \frac{r}{R_0} \right) \right) \right),
\end{aligned} \tag{A.272}
$$

$$
\begin{aligned}
\text{Fig. 9(f5.12)} = & \left( \frac{4}{3} \left( -55 + 9\pi^2 \right) \right) \left( \frac{G^4}{r^5} \frac{\vec{S}_1}{m_1} \cdot \; \vec{v}_2 \times \vec{n} \, m_1^2 m_2^3 \right) \\
& - \frac{40}{3} \left( \frac{G^4}{r^5} \frac{\vec{S}_1}{m_1} \cdot \; \vec{v}_2 \times \vec{n} \, m_1^2 m_2^3 \; \left( \frac{1}{d-3} - 4 \ln \left( \frac{r}{R_0} \right) \right) \right),
\end{aligned} \tag{A.273}
$$

$$
\begin{aligned}
\text{Fig. 9(f5.13)} = & \frac{116}{15} \left( \frac{G^4}{r^5} \; \frac{\vec{S}_1}{m_1} \cdot \vec{v}_1 \times \vec{n} \, m_1^3 m_2^2 \; \left( \frac{1}{d-3} - 4 \ln \left( \frac{r}{R_0} \right) \right) \right) \\
& + \frac{624}{25} \left( \frac{G^4}{r^5} \frac{\vec{S}_1}{m_1} \cdot \; \vec{v}_1 \times \vec{n} \, m_1^3 m_2^2 \right),
\end{aligned} \tag{A.274}
$$

$$
\begin{aligned}
\text{Fig. 9(f5.14)} = & \left( \frac{1}{6} \left( -11 + 3\pi^2 \right) \right) \left( \frac{G^4}{r^5} \frac{\vec{S}_1}{m_1} \cdot \; \vec{v}_1 \times \vec{n} \, m_1^3 m_2^2 \right) \\
& - \frac{1}{3} \left( \frac{G^4}{r^5} \frac{\vec{S}_1}{m_1} \cdot \; \vec{v}_1 \times \vec{n} \, m_1^3 m_2^2 \; \left( \frac{1}{d-3} - 4 \ln \left( \frac{r}{R_0} \right) \right) \right),
\end{aligned} \tag{A.275}
$$

$$
\begin{aligned}
\text{Fig. 9(f5.15)} = & \frac{11}{15} \left( \frac{G^4}{r^5} \; \frac{\vec{S}_1}{m_1} \cdot \vec{v}_1 \times \vec{n} \, m_1^2 m_2^3 \; \left( \frac{1}{d-3} - 4 \ln \left( \frac{r}{R_0} \right) \right) \right) \\
& + \left( \frac{1}{300} \left( 1048 - 75\pi^2 \right) \right) \left( \frac{G^4}{r^5} \frac{\vec{S}_1}{m_1} \cdot \; \vec{v}_1 \times \vec{n} \, m_1^2 m_2^3 \right),
\end{aligned} \tag{A.276}
$$

$$
\begin{aligned}
\text{Fig. 9(f5.16)} = & \left( \frac{G^4}{r^5} \frac{\vec{S}_1}{m_1} \cdot \; \vec{v}_2 \times \vec{n} \, m_1^2 m_2^3 \; \left( \frac{1}{d-3} - 4 \ln \left( \frac{r}{R_0} \right) \right) \right) \\
& + \left( \frac{1}{12} \left( 50 - 3\pi^2 \right) \right) \left( \frac{G^4}{r^5} \; \frac{\vec{S}_1}{m_1} \cdot \vec{v}_2 \times \vec{n} \, m_1^2 \; m_2^3 \right),
\end{aligned} \tag{A.277}
$$

$$
\begin{aligned}
\text{Fig. 9(f5.17)} = & -\frac{5}{3} \left( \frac{G^4}{r^5} \; \frac{\vec{S}_1}{m_1} \cdot \vec{v}_1 \times \vec{n} \, m_1^3 m_2^2 \; \left( \frac{1}{d-3} - 4 \ln \left( \frac{r}{R_0} \right) \right) \right) \\
& + \left( \frac{1}{4} \left( 26 - \pi^2 \right) \right) \left( - \left( \frac{G^4}{r^5} \frac{\vec{S}_1}{m_1} \cdot \; \vec{v}_1 \times \vec{n} \, m_1^3 m_2^2 \right) \right) \\
& - \frac{2}{3} \left( \frac{G^4}{r^5} \frac{\vec{S}_1}{m_1} \cdot \; \vec{v}_2 \times \vec{n} \, m_1^3 m_2^2 \; \left( \frac{1}{d-3} - 4 \ln \left( \frac{r}{R_0} \right) \right) \right)
\end{aligned} \tag{A.278}
$$

$$+\left(\frac{1}{4}\left(-8+\pi^2\right)\right)\left(\frac{G^4}{r^5}\ \frac{\vec{S}_1}{m_1}\cdot\vec{v}_2\times\vec{n}\,m_1^3\ m_2^2\right),$$

$$\text{Fig. 10(g1.1)} = -\frac{1}{3}\left(\frac{G^4}{r^5}\ \frac{\vec{S}_1}{m_1}\cdot\vec{v}_1\times\vec{n}\,m_1^2m_2^3\ \left(\frac{1}{d-3}-4\ln\left(\frac{r}{R_0}\right)\right)\right) - \frac{11}{6}\left(\frac{G^4}{r^5}\frac{\vec{S}_1}{m_1}\cdot\ \vec{v}_1\times\vec{n}\,m_1^2m_2^3\right), \tag{A.279}$$

$$\text{Fig. 10(g1.2)} = \frac{4}{105}\left(\frac{G^4}{r^5}\ \frac{\vec{S}_1}{m_1}\cdot\vec{v}_1\times\vec{n}\,m_1^3m_2^2\ \left(\frac{1}{d-3}-4\ln\left(\frac{r}{R_0}\right)\right)\right) + \frac{556}{3675}\left(\frac{G^4}{r^5}\frac{\vec{S}_1}{m_1}\cdot\ \vec{v}_1\times\vec{n}\,m_1^3m_2^2\right), \tag{A.280}$$

$$\text{Fig. 10(g1.3)} = -\frac{16}{105}\left(\frac{G^4}{r^5}\ \frac{\vec{S}_1}{m_1}\cdot\vec{v}_1\times\vec{n}\,m_1^3m_2^2\ \left(\frac{1}{d-3}-4\ln\left(\frac{r}{R_0}\right)\right)\right) - \frac{2504}{3675}\left(\frac{G^4}{r^5}\frac{\vec{S}_1}{m_1}\cdot\ \vec{v}_1\times\vec{n}\,m_1^3m_2^2\right), \tag{A.281}$$

$$\text{Fig. 10(g1.4)} = -\frac{4}{105}\left(\frac{G^4}{r^5}\ \frac{\vec{S}_1}{m_1}\cdot\vec{v}_1\times\vec{n}\,m_1^3m_2^2\ \left(\frac{1}{d-3}-4\ln\left(\frac{r}{R_0}\right)\right)\right) - \frac{556}{3675}\left(\frac{G^4}{r^5}\frac{\vec{S}_1}{m_1}\cdot\ \vec{v}_1\times\vec{n}\,m_1^3m_2^2\right), \tag{A.282}$$

$$\text{Fig. 10(g1.5)} = -\frac{8}{105}\left(\frac{G^4}{r^5}\ \frac{\vec{S}_1}{m_1}\cdot\vec{v}_1\times\vec{n}\,m_1^3m_2^2\ \left(\frac{1}{d-3}-4\ln\left(\frac{r}{R_0}\right)\right)\right) - \frac{272}{3675}\left(\frac{G^4}{r^5}\frac{\vec{S}_1}{m_1}\cdot\ \vec{v}_1\times\vec{n}\,m_1^3m_2^2\right), \tag{A.283}$$

$$\text{Fig. 10(g1.6)} = -\frac{4}{35}\left(\frac{G^4}{r^5}\ \frac{\vec{S}_1}{m_1}\cdot\vec{v}_1\times\vec{n}\,m_1^3m_2^2\ \left(\frac{1}{d-3}-4\ln\left(\frac{r}{R_0}\right)\right)\right) - \frac{1318}{3675}\left(\frac{G^4}{r^5}\frac{\vec{S}_1}{m_1}\cdot\ \vec{v}_1\times\vec{n}\,m_1^3m_2^2\right), \tag{A.284}$$

$$\text{Fig. 10(g1.7)} = 0, \tag{A.285}$$

$$\text{Fig. 10(g1.8)} = -\frac{1}{105}\left(\frac{G^4}{r^5}\ \frac{\vec{S}_1}{m_1}\cdot\vec{v}_1\times\vec{n}\,m_1^3m_2^2\ \left(\frac{1}{d-3}-4\ln\left(\frac{r}{R_0}\right)\right)\right) - \frac{209}{3675}\left(\frac{G^4}{r^5}\frac{\vec{S}_1}{m_1}\cdot\ \vec{v}_1\times\vec{n}\,m_1^3m_2^2\right), \tag{A.286}$$

$$\text{Fig. 10(g1.9)} = \frac{4}{3}\left(\frac{G^4}{r^5}\ \frac{\vec{S}_1}{m_1}\cdot\vec{v}_1\times\vec{n}\,m_1^2m_2^3\ \left(\frac{1}{d-3}-4\ln\left(\frac{r}{R_0}\right)\right)\right) \tag{A.287}$$

$$+\,8\left(\frac{G^4}{r^5}\frac{\vec{S}_1}{m_1}\cdot\ \vec{v}_1\times\vec{n}\,m_1^2m_2^3\right),$$

$$\text{Fig. 10(g1.10)}=\frac{4}{15}\left(\frac{G^4}{r^5}\ \frac{\vec{S}_1}{m_1}\cdot\vec{v}_2\times\vec{n}\,m_1^2m_2^3\ \left(\frac{1}{d-3}-4\ln\left(\frac{r}{R_0}\right)\right)\right)\tag{A.288}$$

$$+\,\frac{118}{75}\left(\frac{G^4}{r^5}\frac{\vec{S}_1}{m_1}\cdot\ \vec{v}_2\times\vec{n}\,m_1^2m_2^3\right),$$

$$\text{Fig. 10(g1.11)}=-\frac{16}{15}\left(\frac{G^4}{r^5}\ \frac{\vec{S}_1}{m_1}\cdot\vec{v}_2\times\vec{n}\,m_1^3m_2^2\ \left(\frac{1}{d-3}-4\ln\left(\frac{r}{R_0}\right)\right)\right)\tag{A.289}$$

$$-\,\frac{184}{25}\left(\frac{G^4}{r^5}\frac{\vec{S}_1}{m_1}\cdot\ \vec{v}_2\times\vec{n}\,m_1^3m_2^2\right),$$

$$\text{Fig. 10(g1.12)}=-\frac{4}{15}\left(\frac{G^4}{r^5}\ \frac{\vec{S}_1}{m_1}\cdot\vec{v}_2\times\vec{n}\,m_1^2m_2^3\ \left(\frac{1}{d-3}-4\ln\left(\frac{r}{R_0}\right)\right)\right)\tag{A.290}$$

$$-\,\frac{268}{75}\left(\frac{G^4}{r^5}\frac{\vec{S}_1}{m_1}\cdot\ \vec{v}_2\times\vec{n}\,m_1^2m_2^3\right),$$

$$\text{Fig. 10(g1.13)}=-\frac{64}{3}\left(\frac{G^4}{r^5}\ \frac{\vec{S}_1}{m_1}\cdot\vec{v}_2\times\vec{n}\,m_1^2m_2^3\ \left(\frac{1}{d-3}-4\ln\left(\frac{r}{R_0}\right)\right)\right)\tag{A.291}$$

$$-\,\frac{224}{3}\left(\frac{G^4}{r^5}\frac{\vec{S}_1}{m_1}\cdot\ \vec{v}_2\times\vec{n}\,m_1^2m_2^3\right),$$

$$\text{Fig. 10(g1.14)}=-\frac{64}{5}\left(\frac{G^4}{r^5}\ \frac{\vec{S}_1}{m_1}\cdot\vec{v}_2\times\vec{n}\,m_1^3m_2^2\ \left(\frac{1}{d-3}-4\ln\left(\frac{r}{R_0}\right)\right)\right)\tag{A.292}$$

$$-\,\frac{3424}{75}\left(\frac{G^4}{r^5}\frac{\vec{S}_1}{m_1}\cdot\ \vec{v}_2\times\vec{n}\,m_1^3m_2^2\right),$$

$$\text{Fig. 10(g1.15)}=\frac{4}{3}\left(\frac{G^4}{r^5}\ \frac{\vec{S}_1}{m_1}\cdot\vec{v}_2\times\vec{n}\,m_1^2m_2^3\ \left(\frac{1}{d-3}-4\ln\left(\frac{r}{R_0}\right)\right)\right)\tag{A.293}$$

$$+\,\frac{14}{3}\left(\frac{G^4}{r^5}\frac{\vec{S}_1}{m_1}\cdot\ \vec{v}_2\times\vec{n}\,m_1^2m_2^3\right),$$

$$\text{Fig. 10(g1.16)}=\frac{1}{3}\left(\frac{G^4}{r^5}\ \frac{\vec{S}_1}{m_1}\cdot\vec{v}_1\times\vec{n}\,m_1^2m_2^3\ \left(\frac{1}{d-3}-4\ln\left(\frac{r}{R_0}\right)\right)\right)\tag{A.294}$$

$$+\,\frac{11}{6}\left(\frac{G^4}{r^5}\frac{\vec{S}_1}{m_1}\cdot\ \vec{v}_1\times\vec{n}\,m_1^2m_2^3\right),$$

$$\text{Fig. 10(g1.17)}=\frac{1}{15}\left(\frac{G^4}{r^5}\ \frac{\vec{S}_1}{m_1}\cdot\vec{v}_2\times\vec{n}\,m_1^3m_2^2\ \left(\frac{1}{d-3}-4\ln\left(\frac{r}{R_0}\right)\right)\right)\tag{A.295}$$

$$+\,\frac{23}{50}\left(\frac{G^4}{r^5}\frac{\vec{S}_1}{m_1}\cdot\ \vec{v}_2\times\vec{n}\,m_1^3m_2^2\right),$$

$$\text{Fig. 10(g1.18)} = \frac{4}{5}\left(\frac{G^4}{r^5}\ \frac{\vec{S}_1}{m_1}\cdot\vec{v}_2\times\vec{n}\, m_1^3 m_2^2\ \left(\frac{1}{d-3}-4\ln\left(\frac{r}{R_0}\right)\right)\right) + \frac{214}{75}\left(\frac{G^4}{r^5}\frac{\vec{S}_1}{m_1}\cdot\ \vec{v}_2\times\vec{n}\, m_1^3 m_2^2\right), \tag{A.296}$$

$$\text{Fig. 10(g1.19)} = \frac{3}{35}\left(\frac{G^4}{r^5}\ \frac{\vec{S}_1}{m_1}\cdot\vec{v}_1\times\vec{n}\, m_1^3 m_2^2\ \left(\frac{1}{d-3}-4\ln\left(\frac{r}{R_0}\right)\right)\right) - \frac{149}{3675}\left(\frac{G^4}{r^5}\frac{\vec{S}_1}{m_1}\cdot\ \vec{v}_1\times\vec{n}\, m_1^3 m_2^2\right), \tag{A.297}$$

$$\text{Fig. 10(g1.20)} = \frac{2}{21}\left(\frac{G^4}{r^5}\ \frac{\vec{S}_1}{m_1}\cdot\vec{v}_1\times\vec{n}\, m_1^3 m_2^2\ \left(\frac{1}{d-3}-4\ln\left(\frac{r}{R_0}\right)\right)\right) + \frac{123}{245}\left(\frac{G^4}{r^5}\frac{\vec{S}_1}{m_1}\cdot\ \vec{v}_1\times\vec{n}\, m_1^3 m_2^2\right), \tag{A.298}$$

$$\text{Fig. 10(g2.1)} = -\frac{4}{3}\left(\frac{G^4}{r^5}\ \frac{\vec{S}_1}{m_1}\cdot\vec{v}_2\times\vec{n}\, m_1 m_2^4\right), \tag{A.299}$$

$$\text{Fig. 10(g2.2)} = \frac{1}{6}\left(\frac{G^4}{r^5}\ \frac{\vec{S}_1}{m_1}\cdot\vec{v}_2\times\vec{n}\, m_1 m_2^4\right), \tag{A.300}$$

$$\text{Fig. 10(g2.3)} = -\frac{2}{9}\left(\frac{G^4}{r^5}\ \frac{\vec{S}_1}{m_1}\cdot\vec{v}_2\times\vec{n}\, m_1^4 m_2\right), \tag{A.301}$$

$$\text{Fig. 10(g2.4)} = \frac{4}{3}\left(\frac{G^4}{r^5}\ \frac{\vec{S}_1}{m_1}\cdot\vec{v}_1\times\vec{n}\, m_1^4 m_2\right), \tag{A.302}$$

$$\text{Fig. 10(g2.5)} = \frac{1}{3}\left(\frac{G^4}{r^5}\ \frac{\vec{S}_1}{m_1}\cdot\vec{v}_1\times\vec{n}\, m_1^4 m_2\right), \tag{A.303}$$

$$\text{Fig. 10(g2.6)} = -\frac{1}{3}\left(\frac{G^4}{r^5}\ \frac{\vec{S}_1}{m_1}\cdot\vec{v}_1\times\vec{n}\, m_1^4 m_2\right), \tag{A.304}$$

$$\text{Fig. 10(g2.7)} = \frac{32}{9}\left(\frac{G^4}{r^5}\ \frac{\vec{S}_1}{m_1}\cdot\vec{v}_1\times\vec{n}\, m_1^4 m_2\right), \tag{A.305}$$

$$\text{Fig. 10(g2.8)} = -\frac{2}{9}\left(\frac{G^4}{r^5}\ \frac{\vec{S}_1}{m_1}\cdot\vec{v}_1\times\vec{n}\, m_1^4 m_2\right), \tag{A.306}$$

$$\text{Fig. 10(g2.9)} = -\frac{4}{9}\left(\frac{G^4}{r^5}\ \frac{\vec{S}_1}{m_1}\cdot\vec{v}_1\times\vec{n}\, m_1^4 m_2\right), \tag{A.307}$$

$$\text{Fig. 10(g2.10)} = \frac{1}{2}\left(\frac{G^4}{r^5}\ \frac{\vec{S}_1}{m_1}\cdot\vec{v}_1\times\vec{n}\, m_1 m_2^4\right), \tag{A.308}$$

$$\text{Fig. 10(g2.11)} = -\frac{5}{18}\left(\frac{G^4}{r^5}\ \frac{\vec{S}_1}{m_1}\cdot\vec{v}_2\times\vec{n}\, m_1 m_2^4\right), \tag{A.309}$$

$$\text{Fig. 10(g3.1)} = -\frac{8}{3}\left(\frac{G^4}{r^5}\ \frac{\vec{S}_1}{m_1}\cdot\vec{v}_2\times\vec{n}\,m_1m_2^4\right), \tag{A.310}$$

$$\text{Fig. 10(g3.2)} = -\frac{4}{9}\left(\frac{G^4}{r^5}\ \frac{\vec{S}_1}{m_1}\cdot\vec{v}_2\times\vec{n}\,m_1^4m_2\right), \tag{A.311}$$

$$\text{Fig. 10(g3.3)} = -\frac{8}{5}\left(\frac{G^4}{r^5}\ \frac{\vec{S}_1}{m_1}\cdot\vec{v}_2\times\vec{n}\,m_1m_2^4\right), \tag{A.312}$$

$$\text{Fig. 10(g3.4)} = -\frac{52}{45}\left(\frac{G^4}{r^5}\ \frac{\vec{S}_1}{m_1}\cdot\vec{v}_2\times\vec{n}\,m_1^4m_2\right), \tag{A.313}$$

$$\text{Fig. 10(g3.5)} = \frac{4}{45}\left(\frac{G^4}{r^5}\ \frac{\vec{S}_1}{m_1}\cdot\vec{v}_1\times\vec{n}\,m_1^4m_2\right), \tag{A.314}$$

$$\text{Fig. 10(g3.6)} = \frac{4}{15}\left(\frac{G^4}{r^5}\ \frac{\vec{S}_1}{m_1}\cdot\vec{v}_1\times\vec{n}\,m_1^4m_2\right), \tag{A.315}$$

$$\text{Fig. 10(g3.7)} = \frac{8}{5}\left(\frac{G^4}{r^5}\ \frac{\vec{S}_1}{m_1}\cdot\vec{v}_2\times\vec{n}\,m_1m_2^4\right), \tag{A.316}$$

$$\text{Fig. 10(g3.8)} = -\frac{4}{45}\left(\frac{G^4}{r^5}\ \frac{\vec{S}_1}{m_1}\cdot\vec{v}_1\times\vec{n}\,m_1^4m_2\right), \tag{A.317}$$

$$\text{Fig. 10(g3.9)} = -128\left(\frac{G^4}{r^5}\frac{\vec{S}_1}{m_1}\cdot\ \vec{v}_2\times\vec{n}\,m_1m_2^4\right), \tag{A.318}$$

$$\text{Fig. 10(g3.10)} = -\frac{208}{15}\left(\frac{G^4}{r^5}\ \frac{\vec{S}_1}{m_1}\cdot\vec{v}_2\times\vec{n}\,m_1^4m_2\right), \tag{A.319}$$

$$\text{Fig. 10(g3.11)} = \frac{64}{9}\left(\frac{G^4}{r^5}\ \frac{\vec{S}_1}{m_1}\cdot\vec{v}_1\times\vec{n}\,m_1^4m_2\right), \tag{A.320}$$

$$\text{Fig. 10(g3.12)} = \frac{16}{5}\left(\frac{G^4}{r^5}\ \frac{\vec{S}_1}{m_1}\cdot\vec{v}_1\times\vec{n}\,m_1^4m_2\right), \tag{A.321}$$

$$\text{Fig. 10(g3.13)} = 8\left(\frac{G^4}{r^5}\frac{\vec{S}_1}{m_1}\cdot\ \vec{v}_2\times\vec{n}\,m_1m_2^4\right), \tag{A.322}$$

$$\text{Fig. 10(g3.14)} = -\frac{4}{9}\left(\frac{G^4}{r^5}\ \frac{\vec{S}_1}{m_1}\cdot\vec{v}_1\times\vec{n}\,m_1^4m_2\right), \tag{A.323}$$

$$\text{Fig. 10(g3.15)} = -\frac{2}{9}\left(\frac{G^4}{r^5}\ \frac{\vec{S}_1}{m_1}\cdot\vec{v}_1\times\vec{n}\,m_1m_2^4\right), \tag{A.324}$$

$$\text{Fig. 10(g3.16)} = -\frac{1}{9}\left(\frac{G^4}{r^5}\ \frac{\vec{S}_1}{m_1}\cdot\vec{v}_1\times\vec{n}\,m_1^4m_2\right), \tag{A.325}$$

$$\text{Fig. 10(g3.17)} = \frac{8}{105}\left(\frac{G^4}{r^5}\ \frac{\vec{S}_1}{m_1}\cdot\vec{v}_1\times\vec{n}\,m_1^4m_2\ \left(\frac{1}{d-3}-4\ln\left(\frac{r}{R_0}\right)\right)\right) \tag{A.326}$$

$$+\frac{2741}{11025}\left(\frac{G^4}{r^5}\frac{\vec{S}_1}{m_1}\cdot\ \vec{v}_1\times\vec{n}\,m_1^4m_2\right),$$

$$\text{Fig. 10(g3.18)} = -\frac{32}{105}\left(\frac{G^4}{r^5}\ \frac{\vec{S}_1}{m_1}\cdot\vec{v}_1\times\vec{n}\,m_1^4m_2\ \left(\frac{1}{d-3}-4\ln\left(\frac{r}{R_0}\right)\right)\right) \tag{A.327}$$

$$-\frac{12644}{11025}\left(\frac{G^4}{r^5}\frac{\vec{S}_1}{m_1}\cdot\ \vec{v}_1\times\vec{n}\,m_1^4m_2\right),$$

$$\text{Fig. 10(g3.19)} = -\frac{8}{105}\left(\frac{G^4}{r^5}\ \frac{\vec{S}_1}{m_1}\cdot\vec{v}_1\times\vec{n}\,m_1^4m_2\ \left(\frac{1}{d-3}-4\ln\left(\frac{r}{R_0}\right)\right)\right) \tag{A.328}$$

$$-\frac{2741}{11025}\left(\frac{G^4}{r^5}\frac{\vec{S}_1}{m_1}\cdot\ \vec{v}_1\times\vec{n}\,m_1^4m_2\right),$$

$$\text{Fig. 10(g3.20)} = \frac{32}{35}\left(\frac{G^4}{r^5}\ \frac{\vec{S}_1}{m_1}\cdot\vec{v}_1\times\vec{n}\,m_1^4m_2\ \left(\frac{1}{d-3}-4\ln\left(\frac{r}{R_0}\right)\right)\right) \tag{A.329}$$

$$+\frac{14552}{11025}\left(\frac{G^4}{r^5}\frac{\vec{S}_1}{m_1}\cdot\ \vec{v}_1\times\vec{n}\,m_1^4m_2\right),$$

$$\text{Fig. 10(g3.21)} = \frac{32}{105}\left(\frac{G^4}{r^5}\ \frac{\vec{S}_1}{m_1}\cdot\vec{v}_1\times\vec{n}\,m_1^4m_2\ \left(\frac{1}{d-3}-4\ln\left(\frac{r}{R_0}\right)\right)\right) \tag{A.330}$$

$$+\frac{2908}{3675}\left(\frac{G^4}{r^5}\frac{\vec{S}_1}{m_1}\cdot\ \vec{v}_1\times\vec{n}\,m_1^4m_2\right),$$

$$\text{Fig. 10(g3.22)} = -\frac{3}{35}\left(\frac{G^4}{r^5}\ \frac{\vec{S}_1}{m_1}\cdot\vec{v}_1\times\vec{n}\,m_1^4m_2\ \left(\frac{1}{d-3}-4\ln\left(\frac{r}{R_0}\right)\right)\right) \tag{A.331}$$

$$-\frac{2431}{22050}\left(\frac{G^4}{r^5}\frac{\vec{S}_1}{m_1}\cdot\ \vec{v}_1\times\vec{n}\,m_1^4m_2\right),$$

$$\text{Fig. 10(g3.23)} = \frac{4}{15}\left(\frac{G^4}{r^5}\ \frac{\vec{S}_1}{m_1}\cdot\vec{v}_1\times\vec{n}\,m_1^4m_2\right), \tag{A.332}$$

$$\text{Fig. 10(g3.24)} = \frac{1}{45}\left(\frac{G^4}{r^5}\ \frac{\vec{S}_1}{m_1}\cdot\vec{v}_1\times\vec{n}\,m_1^4m_2\right), \tag{A.333}$$

$$\text{Fig. 10(g3.25)} = \frac{4}{15}\left(\frac{G^4}{r^5}\ \frac{\vec{S}_1}{m_1}\cdot\vec{v}_1\times\vec{n}\,m_1^4m_2\right), \tag{A.334}$$

$$\text{Fig. 10(g3.26)} = \frac{2}{9}\left(\frac{G^4}{r^5}\ \frac{\vec{S}_1}{m_1}\cdot\vec{v}_2\times\vec{n}\,m_1m_2^4\right), \tag{A.335}$$

$$\text{Fig. 10(g3.27)} = \frac{1}{9}\left(\frac{G^4}{r^5}\ \frac{\vec{S}_1}{m_1}\cdot\vec{v}_1\times\vec{n}\,m_1^4m_2\right), \tag{A.336}$$

$$\text{Fig. 10(g3.28)} = -\frac{2}{21}\left(\frac{G^4}{r^5}\ \frac{\vec{S}_1}{m_1}\cdot\vec{v}_1\times\vec{n}\,m_1^4m_2\ \left(\frac{1}{d-3}-4\ln\left(\frac{r}{R_0}\right)\right)\right) \tag{A.337}$$

$$-\frac{284}{245}\left(\frac{G^4}{r^5}\frac{\vec{S}_1}{m_1}\cdot\ \vec{v}_1\times\vec{n}\, m_1^4 m_2\right),$$

$$\text{Fig. 10(g3.29)} = \frac{9}{35}\left(\frac{G^4}{r^5}\ \frac{\vec{S}_1}{m_1}\cdot\vec{v}_1\times\vec{n}\, m_1^4 m_2\ \left(\frac{1}{d-3}-4\ln\left(\frac{r}{R_0}\right)\right)\right) \quad (A.338)$$

$$+\frac{24163}{22050}\left(\frac{G^4}{r^5}\frac{\vec{S}_1}{m_1}\cdot\ \vec{v}_1\times\vec{n}\, m_1^4 m_2\right)$$

$$\text{Fig. 11(g4.1)} = 0, \quad (A.339)$$

$$\text{Fig. 11(g4.2)} = \frac{4}{15}\left(\frac{G^4}{r^5}\ \frac{\vec{S}_1}{m_1}\cdot\vec{v}_2\times\vec{n}\, m_1^3 m_2^2\ \left(\frac{1}{d-3}-4\ln\left(\frac{r}{R_0}\right)\right)\right) \quad (A.340)$$

$$-\frac{34}{25}\left(\frac{G^4}{r^5}\frac{\vec{S}_1}{m_1}\cdot\ \vec{v}_2\times\vec{n}\, m_1^3 m_2^2\right),$$

$$\text{Fig. 11(g4.3)} = -\frac{2}{3}\left(\frac{G^4}{r^5}\ \frac{\vec{S}_1}{m_1}\cdot\vec{v}_2\times\vec{n}\, m_1^2 m_2^3\ \left(\frac{1}{d-3}-4\ln\left(\frac{r}{R_0}\right)\right)\right) \quad (A.341)$$

$$-\frac{7}{3}\left(\frac{G^4}{r^5}\frac{\vec{S}_1}{m_1}\cdot\ \vec{v}_2\times\vec{n}\, m_1^2 m_2^3\right),$$

$$\text{Fig. 11(g4.4)} = -\frac{12}{5}\left(\frac{G^4}{r^5}\ \frac{\vec{S}_1}{m_1}\cdot\vec{v}_1\times\vec{n}\, m_1^3\ m_2^2\right), \quad (A.342)$$

$$\text{Fig. 11(g4.5)} = -\frac{4}{3}\left(\frac{G^4}{r^5}\ \frac{\vec{S}_1}{m_1}\cdot\vec{v}_1\times\vec{n}\, m_1^2 m_2^3\ \left(\frac{1}{d-3}-4\ln\left(\frac{r}{R_0}\right)\right)\right) \quad (A.343)$$

$$-\frac{16}{3}\left(\frac{G^4}{r^5}\frac{\vec{S}_1}{m_1}\cdot\ \vec{v}_1\times\vec{n}\, m_1^2 m_2^3\right),$$

$$\text{Fig. 11(g4.6)} = -\frac{4}{3}\left(\frac{G^4}{r^5}\ \frac{\vec{S}_1}{m_1}\cdot\vec{v}_1\times\vec{n}\, m_1^2 m_2^3\ \left(\frac{1}{d-3}-4\ln\left(\frac{r}{R_0}\right)\right)\right) \quad (A.344)$$

$$-6\ \left(\frac{G^4}{r^5}\frac{\vec{S}_1}{m_1}\cdot\ \vec{v}_1\times\vec{n}\, m_1^2 m_2^3\right),$$

$$\text{Fig. 11(g4.7)} = -\frac{46}{15}\left(\frac{G^4}{r^5}\ \frac{\vec{S}_1}{m_1}\cdot\vec{v}_2\times\vec{n}\, m_1^3\ m_2^2\right), \quad (A.345)$$

$$\text{Fig. 11(g4.8)} = -\frac{4}{5}\left(\frac{G^4}{r^5}\ \frac{\vec{S}_1}{m_1}\cdot\vec{v}_2\times\vec{n}\, m_1^2 m_2^3\ \left(\frac{1}{d-3}-4\ln\left(\frac{r}{R_0}\right)\right)\right) \quad (A.346)$$

$$-\frac{138}{25}\left(\frac{G^4}{r^5}\frac{\vec{S}_1}{m_1}\cdot\ \vec{v}_2\times\vec{n}\, m_1^2 m_2^3\right),$$

$$\text{Fig. 11(g4.9)} = \frac{2}{3}\left(\frac{G^4}{r^5}\ \frac{\vec{S}_1}{m_1}\cdot\vec{v}_2\times\vec{n}\, m_1^2 m_2^3\ \left(\frac{1}{d-3}-4\ln\left(\frac{r}{R_0}\right)\right)\right) \quad (A.347)$$

$$+\frac{5}{3}\left(\frac{G^4}{r^5}\frac{\vec{S}_1}{m_1}\cdot\ \vec{v}_2\times\vec{n}\,m_1^2m_2^3\right),$$

$$\text{Fig. 11(g4.10)} = -\frac{4}{5}\left(\frac{G^4}{r^5}\ \frac{\vec{S}_1}{m_1}\cdot\vec{v}_1\times\vec{n}\,m_1^3m_2^2\ \left(\frac{1}{d-3}-4\ln\left(\frac{r}{R_0}\right)\right)\right) \tag{A.348}$$

$$-\frac{184}{75}\left(\frac{G^4}{r^5}\frac{\vec{S}_1}{m_1}\cdot\ \vec{v}_1\times\vec{n}\,m_1^3m_2^2\right),$$

$$\text{Fig. 11(g4.11)} = -\frac{32}{3}\left(\frac{G^4}{r^5}\ \frac{\vec{S}_1}{m_1}\cdot\vec{v}_2\times\vec{n}\,m_1^2m_2^3\ \left(\frac{1}{d-3}-4\ln\left(\frac{r}{R_0}\right)\right)\right) \tag{A.349}$$

$$-\frac{80}{3}\left(\frac{G^4}{r^5}\frac{\vec{S}_1}{m_1}\cdot\ \vec{v}_2\times\vec{n}\,m_1^2m_2^3\right),$$

$$\text{Fig. 11(g4.12)} = \frac{64}{5}\left(\frac{G^4}{r^5}\ \frac{\vec{S}_1}{m_1}\cdot\vec{v}_1\times\vec{n}\,m_1^3m_2^2\ \left(\frac{1}{d-3}-4\ln\left(\frac{r}{R_0}\right)\right)\right) \tag{A.350}$$

$$+\frac{2944}{75}\left(\frac{G^4}{r^5}\frac{\vec{S}_1}{m_1}\cdot\ \vec{v}_1\times\vec{n}\,m_1^3m_2^2\right),$$

$$\text{Fig. 11(g4.13)} = -\frac{128}{15}\left(\frac{G^4}{r^5}\ \frac{\vec{S}_1}{m_1}\cdot\vec{v}_2\times\vec{n}\,m_1^3m_2^2\ \left(\frac{1}{d-3}-4\ln\left(\frac{r}{R_0}\right)\right)\right) \tag{A.351}$$

$$-\frac{672}{25}\left(\frac{G^4}{r^5}\frac{\vec{S}_1}{m_1}\cdot\ \vec{v}_2\times\vec{n}\,m_1^3m_2^2\right),$$

$$\text{Fig. 11(g4.14)} = \frac{64}{15}\left(\frac{G^4}{r^5}\ \frac{\vec{S}_1}{m_1}\cdot\vec{v}_1\times\vec{n}\,m_1^3m_2^2\ \left(\frac{1}{d-3}-4\ln\left(\frac{r}{R_0}\right)\right)\right) \tag{A.352}$$

$$+\frac{1088}{75}\left(\frac{G^4}{r^5}\frac{\vec{S}_1}{m_1}\cdot\ \vec{v}_1\times\vec{n}\,m_1^3m_2^2\right),$$

$$\text{Fig. 11(g4.15)} = 4\left(\frac{G^4}{r^5}\frac{\vec{S}_1}{m_1}\cdot\ \vec{v}_1\times\vec{n}\,m_1^3m_2^2\ \left(\frac{1}{d-3}-4\ln\left(\frac{r}{R_0}\right)\right)\right) \tag{A.353}$$

$$+\left(\frac{1}{3}\left(44-3\pi^2\right)\right)\left(\frac{G^4}{r^5}\ \frac{\vec{S}_1}{m_1}\cdot\vec{v}_1\times\vec{n}\,m_1^3\ m_2^2\right)$$

$$-\frac{8}{3}\left(\frac{G^4}{r^5}\ \frac{\vec{S}_1}{m_1}\cdot\vec{v}_2\times\vec{n}\,m_1^3m_2^2\ \left(\frac{1}{d-3}-4\ln\left(\frac{r}{R_0}\right)\right)\right)$$

$$+\left(\frac{1}{3}\left(-20+3\pi^2\right)\right)\left(\frac{G^4}{r^5}\ \frac{\vec{S}_1}{m_1}\cdot\vec{v}_2\times\vec{n}\,m_1^3\ m_2^2\right),$$

$$\text{Fig. 11(g4.16)} = \left(\frac{1}{24}\left(-176+27\pi^{\ 2}\right)\right)\left(\frac{G^4}{r^5}\frac{\vec{S}_1}{m_1}\cdot\ \vec{v}_2\times\vec{n}\,m_1^2m_2^3\right) \tag{A.354}$$

$$-\frac{4}{3}\ \left(\frac{G^4}{r^5}\frac{\vec{S}_1}{m_1}\cdot\ \vec{v}_2\times\vec{n}\,m_1^2m_2^3\ \left(\frac{1}{d-3}-4\ln\left(\frac{r}{R_0}\right)\right)\right),$$

$$\text{Fig. 11(g4.17)} = \frac{40}{3}\left(\frac{G^4}{r^5}\,\frac{\vec{S}_1}{m_1}\cdot\vec{v}_2\times\vec{n}\,m_1^2m_2^3\,\left(\frac{1}{d-3}-4\ln\left(\frac{r}{R_0}\right)\right)\right) \tag{A.355}$$
$$-\left(\frac{4}{3}\left(-55+9\pi^2\right)\right)\left(\frac{G^4}{r^5}\,\frac{\vec{S}_1}{m_1}\cdot\vec{v}_2\times\vec{n}\,m_1^2\,m_2^3\right),$$

$$\text{Fig. 11(g4.18)} = \frac{16}{3}\left(\frac{G^4}{r^5}\,\frac{\vec{S}_1}{m_1}\cdot\vec{v}_2\times\vec{n}\,m_1^3m_2^2\,\left(\frac{1}{d-3}-4\ln\left(\frac{r}{R_0}\right)\right)\right) \tag{A.356}$$
$$-\left(\frac{2}{3}\left(-28+3\pi^2\right)\right)\left(\frac{G^4}{r^5}\,\frac{\vec{S}_1}{m_1}\cdot\vec{v}_2\times\vec{n}\,m_1^3\,m_2^2\right),$$

$$\text{Fig. 11(g4.19)} = \frac{4}{3}\left(\frac{G^4}{r^5}\,\frac{\vec{S}_1}{m_1}\cdot\vec{v}_1\times\vec{n}\,m_1^3m_2^2\,\left(\frac{1}{d-3}-4\ln\left(\frac{r}{R_0}\right)\right)\right) \tag{A.357}$$
$$+\left(\frac{1}{2}\left(10-\pi^2\right)\right)\left(\frac{G^4}{r^5}\,\frac{\vec{S}_1}{m_1}\cdot\vec{v}_1\times\vec{n}\,m_1^3\,m_2^2\right),$$

$$\text{Fig. 11(g4.20)} = \left(\frac{2}{3}\left(34-3\pi^{\,2}\right)\right)\left(-\left(\frac{G^4}{r^5}\,\frac{\vec{S}_1}{m_1}\cdot\vec{v}_1\times\vec{n}\,m_1^3\,m_2^2\right)\right) \tag{A.358}$$
$$-\frac{16}{3}\left(\frac{G^4}{r^5}\,\frac{\vec{S}_1}{m_1}\cdot\vec{v}_1\times\vec{n}\,m_1^3m_2^2\,\left(\frac{1}{d-3}-4\ln\left(\frac{r}{R_0}\right)\right)\right),$$

$$\text{Fig. 11(g4.21)} = \left(\frac{1}{2}\left(10-\pi^2\right)\right)\,\left(-\left(\frac{G^4}{r^5}\frac{\vec{S}_1}{m_1}\cdot\;\vec{v}_1\times\vec{n}\,m_1^3m_2^2\right)\right) \tag{A.359}$$
$$-\frac{4}{3}\,\left(\frac{G^4}{r^5}\frac{\vec{S}_1}{m_1}\cdot\;\vec{v}_1\times\vec{n}\,m_1^3m_2^2\,\left(\frac{1}{d-3}-4\ln\left(\frac{r}{R_0}\right)\right)\right),$$

$$\text{Fig. 11(g4.22)} = -\frac{2}{15}\left(\frac{G^4}{r^5}\,\frac{\vec{S}_1}{m_1}\cdot\vec{v}_2\times\vec{n}\,m_1^2m_2^3\,\left(\frac{1}{d-3}-4\ln\left(\frac{r}{R_0}\right)\right)\right) \tag{A.360}$$
$$-\frac{44}{75}\left(\frac{G^4}{r^5}\frac{\vec{S}_1}{m_1}\cdot\;\vec{v}_2\times\vec{n}\,m_1^2m_2^3\right),$$

$$\text{Fig. 11(g4.23)} = -\frac{1}{15}\left(\frac{G^4}{r^5}\,\frac{\vec{S}_1}{m_1}\cdot\vec{v}_1\times\vec{n}\,m_1^3m_2^2\,\left(\frac{1}{d-3}-4\ln\left(\frac{r}{R_0}\right)\right)\right) \tag{A.361}$$
$$-\frac{22}{75}\left(\frac{G^4}{r^5}\frac{\vec{S}_1}{m_1}\cdot\;\vec{v}_1\times\vec{n}\,m_1^3m_2^2\right),$$

$$\text{Fig. 11(g4.24)} = \frac{1}{6}\left(\frac{G^4}{r^5}\,\frac{\vec{S}_1}{m_1}\cdot\vec{v}_1\times\vec{n}\,m_1^2\,m_2^3\right) \tag{A.362}$$
$$-\frac{1}{15}\left(\frac{G^4}{r^5}\,\frac{\vec{S}_1}{m_1}\cdot\vec{v}_2\times\vec{n}\,m_1^2m_2^3\,\left(\frac{1}{d-3}-4\ln\left(\frac{r}{R_0}\right)\right)\right)$$
$$-\frac{19}{150}\left(\frac{G^4}{r^5}\frac{\vec{S}_1}{m_1}\cdot\;\vec{v}_2\times\vec{n}\,m_1^2m_2^3\right),$$

$$\text{Fig. 11(g4.25)} = -\frac{4}{15}\left(\frac{G^4}{r^5}\,\frac{\vec{S}_1}{m_1}\cdot\vec{v}_1\times\vec{n}\,m_1^3m_2^2\,\left(\frac{1}{d-3}-4\ln\left(\frac{r}{R_0}\right)\right)\right) \tag{A.363}$$
$$-\frac{88}{75}\left(\frac{G^4}{r^5}\frac{\vec{S}_1}{m_1}\cdot\;\vec{v}_1\times\vec{n}\,m_1^3m_2^2\right)$$
$$+\frac{4}{3}\left(\frac{G^4}{r^5}\frac{\vec{S}_1}{m_1}\cdot\;\vec{v}_2\times\vec{n}\,m_1^3m_2^2\,\left(\frac{1}{d-3}-4\ln\left(\frac{r}{R_0}\right)\right)\right)$$
$$+4\left(\frac{G^4}{r^5}\frac{\vec{S}_1}{m_1}\cdot\;\vec{v}_2\times\vec{n}\,m_1^3m_2^2\right),$$

$$\text{Fig. 11(g4.26)} = \frac{1}{15}\left(\frac{G^4}{r^5}\,\frac{\vec{S}_1}{m_1}\cdot\vec{v}_1\times\vec{n}\,m_1^3m_2^2\,\left(\frac{1}{d-3}-4\ln\left(\frac{r}{R_0}\right)\right)\right) \tag{A.364}$$
$$+\frac{22}{75}\left(\frac{G^4}{r^5}\frac{\vec{S}_1}{m_1}\cdot\;\vec{v}_1\times\vec{n}\,m_1^3m_2^2\right),$$

$$\text{Fig. 11(g4.27)} = \frac{2}{15}\left(\frac{G^4}{r^5}\,\frac{\vec{S}_1}{m_1}\cdot\vec{v}_1\times\vec{n}\,m_1^2m_2^3\,\left(\frac{1}{d-3}-4\ln\left(\frac{r}{R_0}\right)\right)\right) \tag{A.365}$$
$$+\frac{44}{75}\left(\frac{G^4}{r^5}\frac{\vec{S}_1}{m_1}\cdot\;\vec{v}_1\times\vec{n}\,m_1^2m_2^3\right),$$

$$\text{Fig. 11(g4.28)} = \frac{7\left(832+75\pi^2\right)}{1200}\,\left(-\left(\frac{G^4}{r^5}\frac{\vec{S}_1}{m_1}\cdot\;\vec{v}_1\times\vec{n}\,m_1^2m_2^3\right)\right) \tag{A.366}$$
$$-\frac{7}{15}\left(\frac{G^4}{r^5}\frac{\vec{S}_1}{m_1}\cdot\;\vec{v}_1\times\vec{n}\,m_1^2m_2^3\,\left(\frac{1}{d-3}-4\ln\left(\frac{r}{R_0}\right)\right)\right),$$

$$\text{Fig. 11(g4.29)} = -\frac{2}{3}\left(\frac{G^4}{r^5}\,\frac{\vec{S}_1}{m_1}\cdot\vec{v}_1\times\vec{n}\,m_1^2m_2^3\,\left(\frac{1}{d-3}-4\ln\left(\frac{r}{R_0}\right)\right)\right) \tag{A.367}$$
$$+\left(\frac{1}{16}\left(-40+7\pi^2\right)\right)\left(\frac{G^4}{r^5}\,\frac{\vec{S}_1}{m_1}\cdot\vec{v}_1\times\vec{n}\,m_1^2\,m_2^3\right)$$
$$+\frac{7}{15}\left(\frac{G^4}{r^5}\,\frac{\vec{S}_1}{m_1}\cdot\vec{v}_2\times\vec{n}\,m_1^2m_2^3\,\left(\frac{1}{d-3}-4\ln\left(\frac{r}{R_0}\right)\right)\right)$$
$$-\left(\frac{1}{600}\left(-2792+375\pi^2\right)\right)\left(\frac{G^4}{r^5}\frac{\vec{S}_1}{m_1}\cdot\;\vec{v}_2\times\vec{n}\,m_1^2m_2^3\right),$$

$$\text{Fig. 11(g5.1)} = \left(\frac{1}{10}\left(136-5\pi^2\right)\right)\left(-\left(\frac{G^4}{r^5}\frac{\vec{S}_1}{m_1}\cdot\;\vec{v}_2\times\vec{n}\,m_1^3m_2^2\right)\right), \tag{A.368}$$

$$\text{Fig. 11(g5.2)} = \left(\frac{1}{6}\left(328-15\pi^2\right)\right)\left(-\left(\frac{G^4}{r^5}\frac{\vec{S}_1}{m_1}\cdot\;\vec{v}_2\times\vec{n}\,m_1^2m_2^3\right)\right) \tag{A.369}$$
$$-\frac{8}{3}\left(\frac{G^4}{r^5}\frac{\vec{S}_1}{m_1}\cdot\;\vec{v}_2\times\vec{n}\,m_1^2m_2^3\,\left(\frac{1}{d-3}-4\ln\left(\frac{r}{R_0}\right)\right)\right),$$

$$\text{Fig. 11(g5.3)} = -\frac{6}{5}\left(\frac{G^4}{r^5}\ \frac{\vec{S}_1}{m_1}\cdot\vec{v}_1\times\vec{n}\,m_1^3m_2^2\ \left(\frac{1}{d-3}-4\ln\left(\frac{r}{R_0}\right)\right)\right) \tag{A.370}$$
$$+\left(\frac{1}{75}\left(-526+75\pi^2\right)\right)\ \left(\frac{G^4}{r^5}\frac{\vec{S}_1}{m_1}\cdot\ \vec{v}_1\times\vec{n}\,m_1^3m_2^2\right)$$
$$+\frac{8}{3}\ \left(\frac{G^4}{r^5}\frac{\vec{S}_1}{m_1}\cdot\ \vec{v}_2\times\vec{n}\,m_1^3m_2^2\ \left(\frac{1}{d-3}-4\ln\left(\frac{r}{R_0}\right)\right)\right)$$
$$+\left(\frac{1}{3}\left(52-3\pi^2\right)\right)\left(\frac{G^4}{r^5}\ \frac{\vec{S}_1}{m_1}\cdot\vec{v}_2\times\vec{n}\,m_1^3\ m_2^2\right),$$

$$\text{Fig. 11(g5.4)} = -48\left(\frac{G^4}{r^5}\ \frac{\vec{S}_1}{m_1}\cdot\vec{v}_1\times\vec{n}\,m_1^2\ m_2^3\right) \tag{A.371}$$
$$-4\left(\frac{G^4}{r^5}\frac{\vec{S}_1}{m_1}\cdot\ \vec{v}_2\times\vec{n}\,m_1^2m_2^3\ \left(\frac{1}{d-3}-4\ln\left(\frac{r}{R_0}\right)\right)\right)$$
$$+\frac{58}{3}\left(\frac{G^4}{r^5}\frac{\vec{S}_1}{m_1}\cdot\ \vec{v}_2\times\vec{n}\,m_1^2m_2^3\right),$$

$$\text{Fig. 11(g5.5)} = \left(\frac{1}{10}\left(144+5\pi^2\right)\right)\ \left(-\left(\frac{G^4}{r^5}\frac{\vec{S}_1}{m_1}\cdot\ \vec{v}_1\times\vec{n}\,m_1^3m_2^2\right)\right) \tag{A.372}$$
$$-4\ \left(\frac{G^4}{r^5}\frac{\vec{S}_1}{m_1}\cdot\ \vec{v}_1\times\vec{n}\,m_1^3m_2^2\ \left(\frac{1}{d-3}-4\ln\left(\frac{r}{R_0}\right)\right)\right),$$

$$\text{Fig. 11(g5.6)} = \left(\frac{1}{150}\left(184+225\pi^2\right)\right)\ \left(-\left(\frac{G^4}{r^5}\frac{\vec{S}_1}{m_1}\cdot\ \vec{v}_1\times\vec{n}\,m_1^3m_2^2\right)\right) \tag{A.373}$$
$$-\frac{56}{15}\ \left(\frac{G^4}{r^5}\frac{\vec{S}_1}{m_1}\cdot\ \vec{v}_1\times\vec{n}\,m_1^3m_2^2\ \left(\frac{1}{d-3}-4\ln\left(\frac{r}{R_0}\right)\right)\right),$$

$$\text{Fig. 11(g5.7)} = \frac{16}{3}\left(\frac{G^4}{r^5}\ \frac{\vec{S}_1}{m_1}\cdot\vec{v}_2\times\vec{n}\,m_1^2m_2^3\ \left(\frac{1}{d-3}-4\ln\left(\frac{r}{R_0}\right)\right)\right) \tag{A.374}$$
$$-\left(\frac{5}{6}\left(32+3\pi^2\right)\right)\left(\frac{G^4}{r^5}\ \frac{\vec{S}_1}{m_1}\cdot\vec{v}_2\times\vec{n}\,m_1^2\ m_2^3\right),$$

$$\text{Fig. 11(g5.8)} = \frac{40}{3}\left(\frac{G^4}{r^5}\ \frac{\vec{S}_1}{m_1}\cdot\vec{v}_2\times\vec{n}\,m_1^3m_2^2\ \left(\frac{1}{d-3}-4\ln\left(\frac{r}{R_0}\right)\right)\right) \tag{A.375}$$
$$-\left(\frac{1}{10}\left(-296+45\pi^2\right)\right)\ \left(\frac{G^4}{r^5}\frac{\vec{S}_1}{m_1}\cdot\ \vec{v}_2\times\vec{n}\,m_1^3m_2^2\right),$$

$$\text{Fig. 11(g5.9)} = -\frac{2}{15}\left(\frac{G^4}{r^5}\ \frac{\vec{S}_1}{m_1}\cdot\vec{v}_1\times\vec{n}\,m_1^3m_2^2\ \left(\frac{1}{d-3}-4\ln\left(\frac{r}{R_0}\right)\right)\right) \tag{A.376}$$
$$+\frac{86}{75}\left(\frac{G^4}{r^5}\frac{\vec{S}_1}{m_1}\cdot\ \vec{v}_1\times\vec{n}\,m_1^3m_2^2\right)$$

$$+\frac{8}{3}\left(\frac{G^4}{r^5}\frac{\vec{S}_1}{m_1}\cdot\ \vec{v}_2\times\vec{n}\,m_1^3m_2^2\ \left(\frac{1}{d-3}-4\ln\left(\frac{r}{R_0}\right)\right)\right)$$

$$+\frac{20}{3}\left(\frac{G^4}{r^5}\frac{\vec{S}_1}{m_1}\cdot\ \vec{v}_2\times\vec{n}\,m_1^3m_2^2\right),$$

$$\text{Fig. 11(g5.10)}=8\left(\frac{G^4}{r^5}\frac{\vec{S}_1}{m_1}\cdot\ \vec{v}_1\times\vec{n}\,m_1^2m_2^3\right) \tag{A.377}$$

$$+4\left(\frac{G^4}{r^5}\ \frac{\vec{S}_1}{m_1}\cdot\vec{v}_2\times\vec{n}\,m_1^2m_2^3\ \left(\frac{1}{d-3}-4\ln\left(\frac{r}{R_0}\right)\right)\right)$$

$$+\frac{14}{3}\left(\frac{G^4}{r^5}\frac{\vec{S}_1}{m_1}\cdot\ \vec{v}_2\times\vec{n}\,m_1^2m_2^3\right),$$

$$\text{Fig. 11(g5.11)}=\frac{40}{3}\left(\frac{G^4}{r^5}\ \frac{\vec{S}_1}{m_1}\cdot\vec{v}_1\times\vec{n}\,m_1^3m_2^2\ \left(\frac{1}{d-3}-4\ln\left(\frac{r}{R_0}\right)\right)\right) \tag{A.378}$$

$$+\frac{604}{15}\left(\frac{G^4}{r^5}\frac{\vec{S}_1}{m_1}\cdot\ \vec{v}_1\times\vec{n}\,m_1^3m_2^2\right),$$

$$\text{Fig. 11(g5.12)}=-\frac{136}{15}\left(\frac{G^4}{r^5}\ \frac{\vec{S}_1}{m_1}\cdot\vec{v}_2\times\vec{n}\,m_1^3m_2^2\ \left(\frac{1}{d-3}-4\ln\left(\frac{r}{R_0}\right)\right)\right) \tag{A.379}$$

$$-\frac{1612}{75}\left(\frac{G^4}{r^5}\frac{\vec{S}_1}{m_1}\cdot\ \vec{v}_2\times\vec{n}\,m_1^3m_2^2\right),$$

$$\text{Fig. 11(g5.13)}=0, \tag{A.380}$$

$$\text{Fig. 11(g5.14)}=32\left(\frac{G^4}{r^5}\frac{\vec{S}_1}{m_1}\cdot\ \vec{v}_1\times\vec{n}\,m_1^2m_2^3\ \left(\frac{1}{d-3}-4\ln\left(\frac{r}{R_0}\right)\right)\right) \tag{A.381}$$

$$+\frac{304}{3}\left(\frac{G^4}{r^5}\frac{\vec{S}_1}{m_1}\cdot\ \vec{v}_1\times\vec{n}\,m_1^2m_2^3\right),$$

$$\text{Fig. 11(g5.15)}=\frac{22}{15}\left(\frac{G^4}{r^5}\ \frac{\vec{S}_1}{m_1}\cdot\vec{v}_1\times\vec{n}\,m_1^3m_2^2\ \left(\frac{1}{d-3}-4\ln\left(\frac{r}{R_0}\right)\right)\right) \tag{A.382}$$

$$+\frac{123}{25}\left(\frac{G^4}{r^5}\frac{\vec{S}_1}{m_1}\cdot\ \vec{v}_1\times\vec{n}\,m_1^3m_2^2\right)$$

$$-\frac{2}{3}\left(\frac{G^4}{r^5}\frac{\vec{S}_1}{m_1}\cdot\ \vec{v}_2\times\vec{n}\,m_1^3m_2^2\ \left(\frac{1}{d-3}-4\ln\left(\frac{r}{R_0}\right)\right)\right)$$

$$-\left(\frac{1}{8}\left(56-3\pi^2\right)\right)\left(\frac{G^4}{r^5}\ \frac{\vec{S}_1}{m_1}\cdot\vec{v}_2\times\vec{n}\,m_1^3\ m_2^2\right),$$

$$\text{Fig. 11(g5.16)}=\left(\frac{1}{120}\left(-1528+165\pi^{\ 2}\right)\right)\left(\frac{G^4}{r^5}\frac{\vec{S}_1}{m_1}\cdot\ \vec{v}_1\times\vec{n}\,m_1^3m_2^2\right) \tag{A.383}$$

$$-\frac{4}{3}\left(\frac{G^4}{r^5}\frac{\vec{S}_1}{m_1}\cdot\ \vec{v}_1\times\vec{n}\,m_1^3m_2^2\ \left(\frac{1}{d-3}-4\ln\left(\frac{r}{R_0}\right)\right)\right),$$

$$\text{Fig. 11(g5.17)} = \left(\frac{1}{120}\left(1136 - 105\pi^2\right)\right)\ \left(-\left(\frac{G^4}{r^5}\frac{\vec{S}_1}{m_1}\cdot\ \vec{v}_1\times\vec{n}\,m_1^2 m_2^3\right)\right) \tag{A.384}$$
$$-\ \frac{2}{3}\ \left(\frac{G^4}{r^5}\frac{\vec{S}_1}{m_1}\cdot\ \vec{v}_1\times\vec{n}\,m_1^2 m_2^3\ \left(\frac{1}{d-3} - 4\ln\left(\frac{r}{R_0}\right)\right)\right),$$

$$\text{Fig. 11(g5.18)} = \left(\frac{1}{120}\left(248 - 15\pi^2\right)\right)\ \left(\frac{G^4}{r^5}\frac{\vec{S}_1}{m_1}\cdot\ \vec{v}_1\times\vec{n}\,m_1^3 m_2^2\right) \tag{A.385}$$
$$+\ \frac{4}{3}\ \left(\frac{G^4}{r^5}\frac{\vec{S}_1}{m_1}\cdot\ \vec{v}_2\times\vec{n}\,m_1^3 m_2^2\ \left(\frac{1}{d-3} - 4\ln\left(\frac{r}{R_0}\right)\right)\right)$$
$$-\left(\frac{1}{12}\left(-128 + 15\pi^2\right)\right)\ \left(\frac{G^4}{r^5}\frac{\vec{S}_1}{m_1}\cdot\ \vec{v}_2\times\vec{n}\,m_1^3 m_2^2\right),$$

$$\text{Fig. 11(g5.19)} = \frac{2}{3}\left(\frac{G^4}{r^5}\ \frac{\vec{S}_1}{m_1}\cdot\vec{v}_1\times\vec{n}\,m_1^2 m_2^3\ \left(\frac{1}{d-3} - 4\ln\left(\frac{r}{R_0}\right)\right)\right) \tag{A.386}$$
$$-\left(\frac{1}{24}\left(-128 + 15\pi^2\right)\right)\ \left(\frac{G^4}{r^5}\frac{\vec{S}_1}{m_1}\cdot\ \vec{v}_1\times\vec{n}\,m_1^2 m_2^3\right)$$
$$+\left(\frac{1}{60}\ \left(248 - 15\pi^2\right)\right)\left(\frac{G^4}{r^5}\ \frac{\vec{S}_1}{m_1}\cdot\vec{v}_2\times\vec{n}\,m_1^2\ m_2^3\right),$$

$$\text{Fig. 11(g5.20)} = \frac{2}{15}\left(\frac{G^4}{r^5}\ \frac{\vec{S}_1}{m_1}\cdot\vec{v}_1\times\vec{n}\,m_1^3 m_2^2\ \left(\frac{1}{d-3} - 4\ln\left(\frac{r}{R_0}\right)\right)\right) \tag{A.387}$$
$$-\left(\frac{1}{75}\left(146 + 75\pi^2\right)\right)\ \left(\frac{G^4}{r^5}\frac{\vec{S}_1}{m_1}\cdot\ \vec{v}_1\times\vec{n}\,m_1^3 m_2^2\right),$$

$$\text{Fig. 11(g5.21)} = \frac{26}{15}\left(\frac{G^4}{r^5}\ \frac{\vec{S}_1}{m_1}\cdot\vec{v}_1\times\vec{n}\,m_1^3 m_2^2\ \left(\frac{1}{d-3} - 4\ln\left(\frac{r}{R_0}\right)\right)\right) \tag{A.388}$$
$$+\left(\frac{19}{150}\left(416 - 25\pi^2\right)\right)\ \left(\frac{G^4}{r^5}\frac{\vec{S}_1}{m_1}\cdot\ \vec{v}_1\times\vec{n}\,m_1^3 m_2^2\right)$$
$$+\left(\frac{1}{24}\ \left(920 - 67\pi^2\right)\right)\left(-\left(\frac{G^4}{r^5}\ \frac{\vec{S}_1}{m_1}\cdot\vec{v}_2\times\vec{n}\,m_1^3\ m_2^2\right)\right).$$
